# Supplementary material for: Asymptotic analysis and design of linear elastic shell lattice metamaterials
Source: arXiv:2506.18910 source file (2025-05-19)
Supplement: Supplementary file 1 [file Supplementary.pdf]

# Supplementary Material: Asymptotic analysis and design of linear elastic shell lattice metamaterials

DI ZHANG, University of Science and Technology of China, China

LIGANG LIU\*, University of Science and Technology of China, China

## ACM Reference Format:

Di Zhang and Ligang Liu. 2025. Supplementary Material: Asymptotic analysis and design of linear elastic shell lattice metamaterials. *ACM Trans. Graph.* 44, 4 (August 2025), 15 pages. <https://doi.org/10.1145/3730888>

## 1 Homogenization

Suppose the RVE of the lattice metamaterial is  $Y := [-1, 1]$ , the solid region within  $Y$  is denoted as  $\Omega \subset Y$ . The traditional form of cell problem in homogenization method is given as follows [Panetta et al. 2015]

$$\begin{cases} -\nabla \cdot (\mathbf{C} : [\varepsilon(\mathbf{u}) + \varepsilon]) = 0 & \text{in } \Omega, \\ \hat{\mathbf{n}} \cdot (\mathbf{C} : [\varepsilon(\mathbf{u}) + \varepsilon]) = 0 & \text{on } \partial\Omega \setminus \partial Y, \\ \mathbf{u} \text{ Y-periodic} \\ \int_{\omega} \mathbf{u} \, dx = 0 \end{cases} \quad (1)$$

where  $\mathbf{C}$  is the elastic tensor of the base material;  $\varepsilon(\mathbf{u})$  denotes the strain induced by  $\mathbf{u}$ ;  $\varepsilon$  signifies the macro-strain. Since the periodic boundary condition complicates the analysis, we identify  $Y$  as 3-torus  $\mathbb{T}^3 := \mathbb{R}^3 / (2\mathbb{Z})^3$  through the following isometric map

$$\tau : \mathbb{R}^3 \rightarrow \mathbb{Z}^3, (x, y, z) \mapsto (\bar{x}, \bar{y}, \bar{z})$$

where  $\bar{x} = x + 2\mathbb{Z}$ , same as  $\bar{y}, \bar{z}$ . Accordingly, the region  $\Omega$  is identified as the region  $\tilde{\Omega} := \tau(\Omega) \subset \mathbb{T}^3$ . In this way, the periodic boundary condition is satisfied inherently [Allaire 2002]. Besides, the zero translation constrain in (1) is not sufficient to guarantee a unique solution in special cases. For example, rotation along  $x$ -axis does not change the strain if  $\Omega$  is a cylindrical shell parallel to  $x$ -axis. Therefore, we replace this constrain as  $\mathbf{u} \in \mathbf{Rig}^\perp$ , where  $\mathbf{Rig}$  denotes the space of rigid motion and the orthogonal complement is in the sense of  $L^2(\tilde{\Omega})$  inner product. Through integration by parts, the cell problem (1) finally becomes finding  $\mathbf{u} \in \mathbf{V}_\#(\tilde{\Omega})$ , such that

$$\int_{\tilde{\Omega}} \varepsilon(\mathbf{u}) : \mathbb{C} : \varepsilon(\mathbf{v}) = - \int_{\tilde{\Omega}} \varepsilon : \mathbb{C} : \varepsilon(\mathbf{v}), \quad \forall \mathbf{v} \in \mathbf{V}_\#(\tilde{\Omega}), \quad (2)$$

where the function space is defined as

$$\mathbf{V}_\#(\tilde{\Omega}) = \mathbf{H}^1(\tilde{\Omega}) \cap \mathbf{Rig}^\perp$$

\*Corresponding author.

Authors' Contact Information: Di Zhang, zhd9702@mail.ustc.edu.cn, University of Science and Technology of China, Hefei, China; Ligang Liu, University of Science and Technology of China, Hefei, China, lgliu@ustc.edu.cn.

Permission to make digital or hard copies of all or part of this work for personal or classroom use is granted without fee provided that copies are not made or distributed for profit or commercial advantage and that copies bear this notice and the full citation on the first page. Copyrights for components of this work owned by others than the author(s) must be honored. Abstracting with credit is permitted. To copy otherwise, or republish, to post on servers or to redistribute to lists, requires prior specific permission and/or a fee. Request permissions from [permissions@acm.org](mailto:permissions@acm.org).

© 2025 Copyright held by the owner/author(s). Publication rights licensed to ACM.

ACM 1557-7368/2025/8-ART

<https://doi.org/10.1145/3730888>

and the notation  $\mathbf{H}^1(\tilde{\Omega}) := H^1(\tilde{\Omega}) \times H^1(\tilde{\Omega}) \times H^1(\tilde{\Omega})$  denotes the vector Sobolev space on  $\tilde{\Omega}$ . Note that this variational equation is equivalent to the following problem:

$$\arg \min_{\mathbf{u} \in \mathbf{V}_\#(\tilde{\Omega})} I_{\tilde{\Omega}}(\mathbf{u}; \varepsilon)$$

where

$$I_{\tilde{\Omega}}(\mathbf{u}; \varepsilon) := \frac{1}{|Y|} \int_{\tilde{\Omega}} (\varepsilon(\mathbf{u}) + \varepsilon) : \mathbb{C} : (\varepsilon(\mathbf{u}) + \varepsilon).$$

The stiffness of lattice  $\tilde{\Omega}$  under strain  $\varepsilon$  is evaluated by

$$E(\tilde{\Omega}; \varepsilon) = \min_{\mathbf{u} \in \mathbf{V}_\#(\tilde{\Omega})} I_{\tilde{\Omega}}(\mathbf{u}; \varepsilon) \quad (3)$$

## 2 Shell lattice metamaterial

We consider a closed smooth 2-manifold  $\tilde{\omega}$  isometrically embedded in  $\mathbb{T}^3$ , which serves as the middle surface of the shell. As  $\tilde{\omega}$  is compact, there exist finite charts  $\{(S_i, \boldsymbol{\psi}_i)\}_{i \in I}$  covering  $\tilde{\omega}$ , where  $\boldsymbol{\psi}_i : S_i \rightarrow \mathcal{U}_i$  is a map from a open set  $S_i \subset \tilde{\omega}$  to the parameter domain  $\mathcal{U}_i \subset \mathbb{R}^2$  and  $I$  is a finite index set. We suppose all  $\mathcal{U}_i$  are bounded in  $\mathbb{R}^2$  and  $\boldsymbol{\psi}_i$  are continuous to boundary of  $\mathcal{U}_i$ , w.l.o.g. Then we construct the shell as a 3-manifold embedded in  $\mathbb{T}^3$  by offsetting  $\tilde{\omega}$  normally on both sides by a small distance. This can be formally stated as the following lemma

LEMMA 1. For sufficiently small<sup>1</sup>  $\epsilon$ , the shell lattice is the subset

$$\tilde{\Omega}^\epsilon := \{\mathbf{x} \in \mathbb{T}^3 : \mathbf{x} = \mathbf{y} + x_3 \mathbf{n}(\mathbf{y}), x_3 \in (-\epsilon, \epsilon), \mathbf{y} \in \tilde{\omega}\},$$

where  $\mathbf{n}(\mathbf{y})$  denotes the normal vector of  $\tilde{\omega}$  at  $\mathbf{y} \in \tilde{\omega}$ . Moreover, it is a smooth manifold embedded in  $\mathbb{T}^3$  with charts  $(B_i^\epsilon, \Phi_i^\epsilon)_{i \in I}$  given by

$$\begin{aligned} B_i^\epsilon &= \{\mathbf{x} \in \mathbb{T}^3 : \mathbf{x} = \mathbf{y} + x_3 \mathbf{n}(\mathbf{y}), x_3 \in (-\epsilon, \epsilon), \mathbf{y} \in S_i\} \\ \Phi_i^\epsilon : B_i^\epsilon &\rightarrow \mathcal{V}_i^\epsilon, \mathbf{y} + x_3 \mathbf{n}(\mathbf{y}) \mapsto (\boldsymbol{\psi}_i(\mathbf{y}), x_3) \end{aligned}$$

where  $\mathcal{V}_i^\epsilon := \mathcal{U}_i \times (-\epsilon, \epsilon)$ .

As above lemma is clear, the proof is omitted.

To conduct the asymptotic analysis as  $\epsilon$  approaches zero, we utilize the native curvilinear coordinates on shell. These curvilinear coordinates rely on the chart of the middle surface. However, covering the middle surface  $\tilde{\omega}$  with a single chart is infeasible due to its non-trivial topology. Therefore, we partition the middle surface  $\tilde{\omega}$  into several disjoint patches  $\{\tilde{\omega}_i\}$ . We suppose  $\tilde{\omega}_i$  is covered by chart  $(S_i, \boldsymbol{\psi}_i)$ . The parametric domain for  $\tilde{\omega}_i$  is denoted as  $U_i := \boldsymbol{\psi}_i(\tilde{\omega}_i)$ . It follows that  $\tilde{\omega}_i \subset S_i$  and  $U_i \subset \mathcal{U}_i$ . Subsequently, we split the shell along normal direction from the cut locus on the mid-surface. The split patches constitutes the partition of  $\tilde{\Omega}^\epsilon$ , denoted as  $\{\tilde{\Omega}_i^\epsilon\}$ , and the corresponding chart of each  $\tilde{\Omega}_i^\epsilon$  is  $(B_i^\epsilon, \Phi_i^\epsilon)$ . We denote  $\Omega_i^\epsilon := \Phi_i^\epsilon(\tilde{\Omega}_i^\epsilon)$ .

<sup>1</sup>Hereafter, sufficiently small  $\epsilon$  means there exist  $\epsilon_0$ , such that the conclusion is true when  $0 < \epsilon \leq \epsilon_0$ .

Then we have  $\tilde{\Omega}_i^\epsilon \subset B_i^\epsilon$  and  $\Omega_i^\epsilon = \Phi_i^\epsilon(\tilde{\Omega}_i^\epsilon) = U_i \times (-\epsilon, \epsilon) \subset \mathcal{V}_i^\epsilon$ . See the illustration in Fig. 1.

For each chart of the shell, we define the related geometry symbols, mostly borrowed from [Ciarlet and Lods 1996; Ciarlet et al. 1996]. For brevity, we omit the index of the chart in certain cases, and the symbols are defined and referenced on the chart indicated by the context. We adopt the following conventions throughout this article:

- **Greek indices (except subscript of chart) and exponents (excluding  $\epsilon$ ) are drawn from the set  $\{1, 2\}$ .**
- **Latin indices and exponents (except when explicitly specified, such as when used for indexing sequences) are selected from the set  $\{1, 2, 3\}$ .**

For each chart  $(B_m^\epsilon, \Phi_m^\epsilon)$ , its parameterization  $\mathbf{r}_m^\epsilon := (\Phi_m^\epsilon)^{-1}$  is

$$\mathbf{r}_m^\epsilon : \Omega_m^\epsilon \rightarrow \tilde{\Omega}_m^\epsilon, (x_1, x_2, x_3) \mapsto \mathbf{r}_m(x_1, x_2) + x_3 \mathbf{n}(x_1, x_2)$$

where  $\Omega_m^\epsilon = U_m \times (-\epsilon, \epsilon)$  and  $\mathbf{r}_m := \psi_m^{-1}$ . We denote the tangent vector of the surface as

$$\mathbf{a}_\alpha = \partial_\alpha \mathbf{r}_m,$$

which are linearly independent on  $U_m$ . They form the covariant basis of the tangent plane to the surface  $\tilde{\omega}$ . The two vectors  $\mathbf{a}^\alpha$ ,  $\alpha = 1, 2$  of the same tangent plane defined by the relation

$$\mathbf{a}^\alpha \cdot \mathbf{a}_\beta = \delta_\beta^\alpha$$

constitute its contravariant basis. We also define the unit vector

$$\mathbf{a}_3 = \mathbf{a}^3 := \mathbf{n}$$

which is the normal vector across  $\tilde{\omega}$ .

Then we define the *first fundamental form*, also known as the metric tensor,  $(a_{\alpha\beta})$  or  $(a^{\alpha\beta})$  (in covariant or contravariant components); the *second fundamental form*, also known as the *curvature tensor*,  $(b_{\alpha\beta})$  or  $(b^{\alpha\beta})$  (in covariant or mixed components), and the *Christoffel symbols*  $\Gamma_{\alpha\beta}^\sigma$ , of the surface  $\tilde{\omega}$  by letting:

$$\begin{aligned} a_{\alpha\beta} &:= \mathbf{a}_\alpha \cdot \mathbf{a}_\beta, & a^{\alpha\beta} &:= \mathbf{a}^\alpha \cdot \mathbf{a}^\beta, \\ b_{\alpha\beta} &:= \mathbf{a}^3 \cdot \partial_\beta \mathbf{a}_\alpha, & b_\alpha^\beta &:= a^{\beta\sigma} b_{\sigma\alpha}, \\ \Gamma_{\alpha\beta}^\sigma &:= \mathbf{a}^\sigma \cdot \partial_\beta \mathbf{a}_\alpha. \end{aligned} \quad (4)$$

To describe vector field on  $\tilde{\omega}$  that may not be tangent, we introduce auxiliary definitions

$$a_{\alpha 3} := \mathbf{a}_\alpha \cdot \mathbf{n} = 0, \quad a^{\alpha 3} := \mathbf{a}^\alpha \cdot \mathbf{n} = 0, \quad a^{33} = a_{33} := \mathbf{n} \cdot \mathbf{n} = 1$$

Then we have  $v^i = a^{ij} v_j$  and  $v_i = a_{ij} v^j$  for a vector field  $\mathbf{v} = v_i \mathbf{a}^i$ . We also define the third fundamental form

$$c_{\alpha\beta} := b_\alpha^\sigma b_{\sigma\beta} \quad (5)$$

Note the symmetries:

$$a_{\alpha\beta} = a_{\beta\alpha}, \quad a^{\alpha\beta} = a^{\beta\alpha}, \quad b_{\alpha\beta} = b_{\beta\alpha}, \quad \Gamma_{\alpha\beta}^\sigma = \Gamma_{\beta\alpha}^\sigma.$$

The *volume form* along  $\tilde{\omega}$  is

$$d\tilde{\omega} = \sqrt{a} dx^1 \wedge dx^2,$$

where

$$a := \det(a_{\alpha\beta}) \quad (6)$$

Similarly, the tangent vectors over  $\tilde{\Omega}_m^\epsilon$ ,

$$\mathbf{g}_i^\epsilon := \partial_i \mathbf{r}_m^\epsilon$$

are linearly independent, which form the covariant basis of the tangent space locally, and the three vectors  $\mathbf{g}^{i,\epsilon}$  defined by

$$\mathbf{g}^{j,\epsilon} \cdot \mathbf{g}_i^\epsilon = \delta_i^j$$

form the contravariant basis. We then define the *metric tensor*  $(g_{ij}^\epsilon)$  or  $(g^{ij,\epsilon})$  (in covariant or contravariant components) and the *Christoffel symbols* of  $\tilde{\Omega}^\epsilon$  by letting

$$\begin{aligned} g_{ij}^\epsilon &:= \mathbf{g}_i^\epsilon \cdot \mathbf{g}_j^\epsilon, & g^{ij,\epsilon} &:= \mathbf{g}^{i,\epsilon} \cdot \mathbf{g}^{j,\epsilon}, \\ \Gamma_{ij}^{p,\epsilon} &:= \mathbf{g}^{p,\epsilon} \cdot \partial_j \mathbf{g}_i^\epsilon. \end{aligned} \quad (7)$$

Note the symmetries

$$g_{ij}^\epsilon = g_{ji}^\epsilon, \quad g^{ij,\epsilon} = g^{ji,\epsilon}, \quad \Gamma_{ij}^{p,\epsilon} = \Gamma_{ji}^{p,\epsilon}.$$

The *volume form* on  $\tilde{\Omega}^\epsilon$  is

$$d\tilde{\Omega}^\epsilon := \sqrt{g^\epsilon} dx^1 \wedge dx^2 \wedge dx^3,$$

where

$$g^\epsilon := \det(g_{ij}^\epsilon) \quad (8)$$

The strain tensor and elastic tensor are denoted as

$$\begin{aligned} \varepsilon(\mathbf{u}^\epsilon) &= e_{i||j}^\epsilon(\mathbf{u}^\epsilon) \mathbf{g}_i^\epsilon \otimes \mathbf{g}_j^\epsilon \\ \mathbf{A} &= A^{ijkl,\epsilon} \mathbf{g}_i^\epsilon \otimes \mathbf{g}_j^\epsilon \otimes \mathbf{g}_k^\epsilon \otimes \mathbf{g}_l^\epsilon, \end{aligned}$$

where the components are given by

$$\begin{aligned} e_{i||j}^\epsilon(\mathbf{u}) &:= \frac{1}{2} \left( \partial_i u_j^\epsilon + \partial_j u_i^\epsilon \right) - \Gamma_{ij}^{p,\epsilon} u_p^\epsilon \\ A^{ijkl,\epsilon} &:= \lambda g^{ij,\epsilon} g^{kl,\epsilon} + \mu \left( g^{ik,\epsilon} g^{jl,\epsilon} + g^{il,\epsilon} g^{jk,\epsilon} \right). \end{aligned} \quad (9)$$

Here, we borrow the notation  $\mathbf{A}$  from [Ciarlet and Lods 1996] to denote the elastic tensor on shell.

We define  $\hat{v}_i$  ( $\hat{v}^i$ ) as the covariant (contravariant) component of vector field  $\mathbf{v}$  under the standard basis  $\{\mathbf{e}^i\}$ , that is

$$\hat{v}_i = \mathbf{e}_i \cdot \mathbf{v}, \quad \hat{v}^i = \mathbf{e}^i \cdot \mathbf{v}$$

As  $\{\mathbf{e}^i\}$  are orthonormal basis and  $\mathbf{e}^i = \mathbf{e}_i$ , we know  $\hat{v}_i = \hat{v}^i$ .

We can transform the components of the vector between curvilinear coordinate system and the standard coordinate system by defining

$$\begin{aligned} \Pi_j^{i,\epsilon} &:= \mathbf{e}^i \cdot \mathbf{g}_j^\epsilon, & \Xi_j^{i,\epsilon} &:= \mathbf{g}^{i,\epsilon} \cdot \mathbf{e}_j, \text{ on } \tilde{\Omega}_m^\epsilon \\ \Pi_j^i &:= \mathbf{e}^i \cdot \mathbf{a}_j, & \Xi_j^i &:= \mathbf{a}^i \cdot \mathbf{e}_j, \text{ on } \tilde{\omega}_m \end{aligned} \quad (10)$$

then we have

$$v_i^\epsilon = \hat{v}_j \Pi_j^{i,\epsilon}, \quad \hat{v}_i = v_j^\epsilon \Xi_j^{i,\epsilon}$$

where  $v_i^\epsilon$  is the covariant component of  $\mathbf{v}$  under basis  $\{\mathbf{g}_i^\epsilon\}$ .

With these notations, the macro-strain  $\varepsilon$  can be represented as

$$\varepsilon = e_{ij}^\epsilon \mathbf{g}^{i,\epsilon} \otimes \mathbf{g}^{j,\epsilon}$$

under the curvilinear coordinate system, where  $e_{ij}^\epsilon = \varepsilon_{kl} \Pi_i^{k,\epsilon} \Pi_j^{l,\epsilon}$ .

**REMARK 1.** As we have assumed that each chart map  $\psi_m$  is continuous to the boundary of  $\mathcal{U}_m$ , all the functions defined in (4), (5), and (6) are continuous to the boundary of  $\mathcal{U}_m$  and thus bounded. Accordingly, the functions defined in (7), (8), and (10) are also continuous to the boundary of  $\mathcal{V}_m^\epsilon$  and bounded.

The difference between the components under two sets of basis  $(\{\mathbf{g}_i^\epsilon\})$  and  $(\{\mathbf{e}_i\})$  is that for a vector field  $\mathbf{v}$  defined on  $\tilde{\Omega}^\epsilon$ , the component

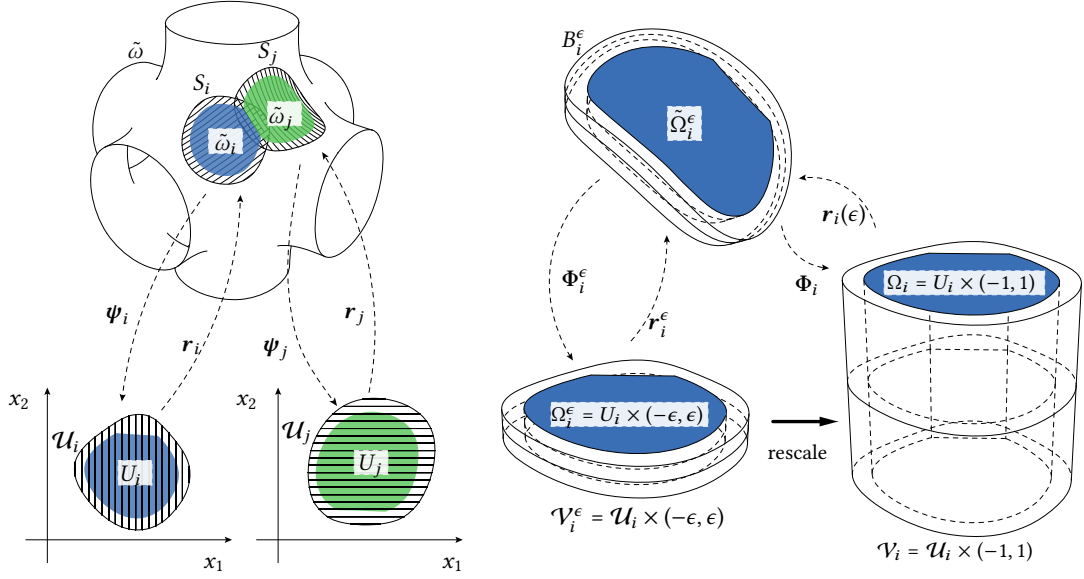

Fig. 1. Illustration of the chart and parameterization.

$\hat{v}_i = \mathbf{e}_i \cdot \mathbf{v}$  is globally defined as it is the dot product of two globally defined vector field, while  $v_i^\epsilon = \mathbf{g}_i^\epsilon \cdot \mathbf{v}$  is only locally defined because the tangent vector  $\mathbf{g}_i^\epsilon$  relies on specific chart. This distinction also holds for the contravariant components  $\hat{v}^i$  and  $v^{i,\epsilon}$ .

## 2.1 Rescaled parameter domain

We eliminate the dependence of the parameter domain on  $\epsilon$  by rescaling it along the normal direction to facilitate asymptotic analysis (Figure 1). This can be done by defining a new chart  $(B_i^\epsilon, \Phi_i)$  as

$$\Phi_i : B_i^\epsilon \rightarrow \mathcal{V}_i, \mathbf{y} + x_3 \mathbf{n} \mapsto \left( \psi_i(\mathbf{y}), \frac{x_3}{\epsilon} \right)$$

where

$$\mathcal{V}_i := \mathcal{U}_i \times (-1, 1).$$

After rescaling, the domain  $\Omega_m^\epsilon = U_m \times (-\epsilon, \epsilon)$  becomes  $\Omega_m := U_m \times (-1, 1)$  accordingly. Then the parameterization on the rescaled domain, denoted as  $\mathbf{r}_i(\epsilon) = \Phi_i^{-1}$ , becomes

$$\mathbf{r}_i(\epsilon) : \mathcal{V}_i \rightarrow B_i^\epsilon, (y, x_3) \mapsto \mathbf{r}_i^\epsilon(y, \epsilon x_3)$$

These notations are illustrated in Fig. 1 for clarity.

We associate a function  $f(\epsilon)$  defined on the rescaled domain with the scalar function  $f^\epsilon$  defined on the original domain by

$$f(\epsilon)(x_1, x_2, x_3) := f^\epsilon(x_1, x_2, \epsilon x_3). \quad (11)$$

We consistently use this notation to define other symbols on the rescaled domain (See Tab. 1).

## 3 Preliminary

We first introduce several preliminary results that are will be used in the subsequent analysis. We denote the Sobolev norm [Hebey 1996] of a function  $f$  over  $\tilde{\Omega}^\epsilon$  as

$$\|f\|_{H^1(\tilde{\Omega}^\epsilon)} = \left( \int_{\tilde{\Omega}^\epsilon} |f|^2 + |\nabla f|^2 d\tilde{\Omega}^\epsilon \right)^{1/2}$$

Table 1. Symbol correspondences before and after rescaling. The first column denotes the evaluation of these functions on middle surface.

| Mid. surf.              | Bef. Res.                                         | Aft. Res.                                         | Description                                                                                                       |
|-------------------------|---------------------------------------------------|---------------------------------------------------|-------------------------------------------------------------------------------------------------------------------|
| $v^i / v_i$             | $v^{i,\epsilon} / v_i^\epsilon$                   | $v^i(\epsilon) / v_i(\epsilon)$                   | Components of vector field $\mathbf{v}$ under basis $\{\mathbf{g}_{i,\epsilon}\} / \{\mathbf{g}^{i,\epsilon}\}$ . |
| $\hat{v}^i / \hat{v}_i$ | $\hat{v}^{i,\epsilon} / \hat{v}_i^\epsilon$       | $\hat{v}^i(\epsilon) / \hat{v}_i(\epsilon)$       | Components of vector field $\mathbf{v}$ under basis $\{\mathbf{e}_i\} / \{\mathbf{e}^i\}$ .                       |
| $\Gamma_{ij}^p$         | $A^{ijkl,\epsilon}$<br>$\Gamma_{ij}^{p,\epsilon}$ | $A^{ijkl}(\epsilon)$<br>$\Gamma_{ij}^p(\epsilon)$ | Components of elastic tensor.<br>Christoffel symbol                                                               |
|                         | $e_{i  j}^\epsilon(\mathbf{u})$                   | $e_{i  j}(\epsilon)(\mathbf{u})$                  | Strain components induced by vector field $\mathbf{u}$ .                                                          |
| $a_{ij} / a^{ij}$       | $g_{ij}^\epsilon / g^{ij,\epsilon}$               | $g_{ij}(\epsilon) / g^{ij}(\epsilon)$             | Components of metric.                                                                                             |
| $e_{ij}$                | $e_{ij}^\epsilon$                                 | $e_{ij}(\epsilon)$                                | macro-strain components                                                                                           |
| $a$                     | $g^\epsilon$                                      | $g(\epsilon)$                                     | Coefficient of volume form.                                                                                       |
| $\Pi_j^i$               | $\Pi_j^{i,\epsilon}$                              | $\Pi_j^i(\epsilon)$                               | Transformation matrix from basis $\{\mathbf{e}_i\}$ to basis $\{\mathbf{g}_i^\epsilon\}$ .                        |
| $\Xi_j^i$               | $\Xi_j^{i,\epsilon}$                              | $\Xi_j^i(\epsilon)$                               | Transformation matrix from basis $\{\mathbf{g}_i^\epsilon\}$ to basis $\{\mathbf{e}_i\}$ .                        |

where  $|\nabla f|$  is the length of the gradient of  $f$ , which can be computed on local coordinates as

$$|\nabla f|^2 = g^{ij} \partial_i f \partial_j f.$$

Here,  $g^{ij}$  is the metric tensor on local chart; The Sobolev norm of a function  $h$  defined on a parameter domain  $\Omega_m \subset \mathbb{R}^3$  is denoted as

$$\|h\|_{0,\Omega_m} = \left( \int_{\Omega_m} h^2 \right)^{1/2}, \quad \|h\|_{1,\Omega_m} = \left( \int_{\Omega_m} h^2 + |\nabla h|^2 \right)^{1/2}$$

which are the  $L^2(\Omega_m)$  and  $H^1(\Omega_m)$  norm, respectively. The analogical definition also holds for  $\|\cdot\|_{0,U_m}$  and  $\|\cdot\|_{1,U_m}$ . When consider the convergence of functions in Sobolev space, we adopt the following convention

- Symbol ‘ $\lesssim$ ’ signifies ‘less than or equal up to a constant’.
- Symbols ‘ $\rightharpoonup$ ’ and ‘ $\rightarrow$ ’ denote weak and strong convergence, respectively.
- Symbols  $\mathcal{C}^\infty(\Omega_m)$  and  $\mathcal{D}(\Omega_m)$  represent the space of smooth functions and smooth functions with compact support, respectively.

We first derive some fundamental results on the geometry quantities defined in Section 2. These results are used in Section 4 to prove our convergence theorem. Based on the definitions, we can immediately get the following relations

LEMMA 2. On each chart  $(B_m^\epsilon, \Phi_m)$ , define the symbols on the rescaled domain according to (11), then we have

$$\mathbf{g}_\alpha(\epsilon) = \mathbf{a}_\alpha - \epsilon x_3 b_\alpha^\beta \mathbf{a}_\beta \quad (12)$$

$$\mathbf{g}^\alpha(\epsilon) = \mathbf{a}^\alpha + \epsilon x_3 b_\sigma^\alpha \mathbf{a}^\sigma + R_\theta^\alpha(\epsilon) \mathbf{a}^\theta \quad (13)$$

$$\mathbf{g}^3(\epsilon) = \mathbf{g}_3(\epsilon) = \mathbf{n} \quad (14)$$

$$g_{\alpha\beta}(\epsilon) = a_{\alpha\beta} - 2\epsilon x_3 b_{\alpha\beta} + \epsilon^2 x_3 b_\alpha^\theta b_{\theta\beta} \quad (15)$$

$$g^{\alpha\beta}(\epsilon) = a^{\alpha\beta} + 2\epsilon x_3 b^{\alpha\beta} + O(\epsilon^2) \quad (16)$$

$$g^{i3}(\epsilon) = g_{i3}(\epsilon) = 0 \quad (17)$$

$$g^{33}(\epsilon) = g_{33}(\epsilon) = 1 \quad (18)$$

$$\sqrt{g(\epsilon)} = (1 - 2H\epsilon x_3 + K\epsilon^2 x_3^2) \sqrt{a} \quad (19)$$

$$0 < a_0 \leq a, \quad 0 < a_0 \leq g(\epsilon) \quad (20)$$

$$a^{\alpha\beta} t_\alpha t_\beta \geq C \sum_\alpha |t_\alpha|^2, \quad g^{ij}(\epsilon) t_i t_j \geq C \sum_i |t_i|^2 \quad (21)$$

$$\Pi_\alpha^i(\epsilon) = \mathbf{e}^i \cdot \mathbf{g}_\alpha(\epsilon) = \Pi_\alpha^i - \epsilon x_3 b_\alpha^\beta \Pi_\beta^i, \quad \Pi_3^i(\epsilon) = \Pi_3^i \quad (22)$$

$$\Xi_i^\alpha(\epsilon) = \mathbf{g}^\alpha(\epsilon) \cdot \mathbf{e}_i = \Xi_i^\alpha + \epsilon x_3 b_\theta^\alpha \Xi_i^\theta + R_\theta^\alpha(\epsilon) \Xi_i^\theta, \quad \Xi_i^3(\epsilon) = \Xi_i^3 \quad (23)$$

$$\Pi_j^i(\epsilon) \Xi_k^j(\epsilon) = \Pi_j^i \Xi_k^j = \delta_k^i \quad (24)$$

for sufficiently small  $\epsilon$  and some constant  $a_0, C > 0$  independent of  $\epsilon$ . Here, the notation  $H$  and  $K$  denotes the mean curvature and Gauss curvature, respectively, and  $R_\theta^\alpha(\epsilon)$  in (13) satisfies

$$(\delta_\alpha^\beta - \epsilon x_3 b_\alpha^\beta) R_\beta^\theta(\epsilon) = \epsilon^2 x_3^2 b_\alpha^\sigma b_\sigma^\theta, \quad (25)$$

and we have

$$R_\theta^\alpha(\epsilon) \in C^\infty(\mathcal{U}_m), \quad \|R_\theta^\alpha(\epsilon)\|_{1,\infty,\mathcal{U}_m} \lesssim \epsilon^2 \quad (26)$$

for sufficiently small  $\epsilon$ . The norm  $\|\cdot\|_{1,\infty,\mathcal{U}_m}$  is defined as

$$\|f\|_{1,\infty,\mathcal{U}_m} = \sup_{k \leq 1, y \in \mathcal{U}_m} |D^k f(y)|.$$

Here,  $D^k$  denotes  $k$ -th order derivative.

PROOF. (12), (13), (14), (15), (16), (17), (18), (19), (22), (23), and (24) can be obtained through direct computation based on their definition. Note that (25) is derived based on relation  $\mathbf{g}_\alpha(\epsilon) \cdot \mathbf{g}^\beta(\epsilon) = \delta_\alpha^\beta$  and (12). Equations (20) and (21) are derived from the positive definiteness of the metric tensors within the parameter domain and their continuity to the boundary. To show that (26) holds, we notice that the matrix  $(\delta_\alpha^\beta - \epsilon x_3 b_\alpha^\beta)$  (regarding  $\alpha, \beta$  as indices) is a infinitely smooth and positive definite when  $\epsilon$  is sufficiently small. Thus the norm of  $R_\beta^\theta(\epsilon)$  is primarily bounded by the RHS of (25), which is a infinitely smooth function multiplies  $\epsilon^2$ . Then, it becomes clear that (26) holds.  $\square$

Similarly, we have an estimation of the Christoffel symbol and elastic tensor, given in the following lemma

LEMMA 3. On each chart  $(B_m^\epsilon, \Phi_m)$ , we define

$$b_\beta^\sigma|_\alpha := \partial_\alpha b_\beta^\sigma + \Gamma_{\alpha\tau}^\sigma b_\beta^\tau - \Gamma_{\beta\alpha}^\tau b_\tau^\sigma,$$

which is the covariant derivative of second fundamental form, and we let functions on  $\mathcal{U}_m$  be identified with functions defined on  $\mathcal{V}_m$  that is constant w.r.t  $x_3$ . Then we have

$$\left\| \Gamma_{\alpha\beta}^\sigma(\epsilon) - \left( \Gamma_{\alpha\beta}^\sigma - \epsilon x_3 b_\beta^\tau \Gamma_{\alpha\tau}^\sigma \right) \right\|_{0,\infty,\Omega_m} \lesssim \epsilon^2 \quad (27)$$

$$\Gamma_{\alpha\beta}^3(\epsilon) = b_{\alpha\beta} - \epsilon x_3 c_{\alpha\beta}$$

$$\left\| \Gamma_{\alpha 3}^\sigma(\epsilon) + b_\alpha^\sigma + \epsilon x_3 b_\alpha^\tau b_\tau^\sigma \right\|_{0,\infty,\Omega_m} \lesssim \epsilon^2$$

$$\Gamma_{\alpha 3}^3(\epsilon) = \Gamma_{33}^3(\epsilon) = 0 \quad (28)$$

$$\|g(\epsilon) - a\|_{0,\infty,\Omega_m} \lesssim \epsilon$$

$$\|A^{ijkl}(\epsilon) - A^{ijkl}(0)\|_{0,\infty,\Omega_m} \lesssim \epsilon$$

$$A^{\alpha\beta\theta 3}(\epsilon) = A^{\alpha 333}(\epsilon) = 0$$

where

$$A^{\alpha\beta\sigma\tau}(0) := \lambda a^{\alpha\beta} a^{\sigma\tau} + \mu (a^{\alpha\sigma} a^{\beta\tau} + a^{\alpha\tau} a^{\beta\sigma})$$

$$A^{\alpha\beta 33}(0) := \lambda a^{\alpha\beta}, \quad A^{\alpha 333}(0) := \mu a^{\alpha\sigma}, \quad A^{3333}(0) := \lambda + 2\mu$$

$$A^{\alpha\beta\sigma 3}(0) = A^{\alpha 333}(0) := 0$$

and

$$C t_{ij} t_{ij} \leq A^{ijkl}(\epsilon) t_{kl} t_{ij} \quad (29)$$

for some constant  $C > 0$  independent of  $\epsilon$  and symmetric  $t_{ij}$ , when  $\epsilon$  is sufficiently small. Here, the norm  $\|\cdot\|_{0,\infty,\Omega_m}$  is defined as

$$\|f\|_{0,\infty,\Omega_m} = \sup_{x \in \Omega_m} |f(x)|.$$

PROOF. These results are borrowed from Lemma 3.1 in [Ciarlet and Lods 1996]. They can be verified through trivial computation based on Lemma 2, we refer the interested reader to [Ciarlet and Lods 1996] for more details.  $\square$

REMARK 2. From (28), we can see that the components of the strain tensor over the rescaled parameter domain are computed by

$$e_{\alpha\| \beta}(\epsilon)(\mathbf{v}) = \frac{1}{2} (\partial_\alpha v_\beta(\epsilon) + \partial_\beta v_\alpha(\epsilon)) - \Gamma_{\alpha\beta}^p(\epsilon) v_p(\epsilon)$$

$$e_{\alpha\| 3}(\epsilon)(\mathbf{v}) = \frac{1}{2} \left( \partial_\alpha v_3(\epsilon) + \frac{1}{\epsilon} \partial_3 v_\alpha(\epsilon) \right) - \Gamma_{\alpha 3}^\theta(\epsilon) v_\theta(\epsilon)$$

$$e_{3\| 3}(\epsilon)(\mathbf{v}) = \frac{1}{\epsilon} \partial_3 v_3(\epsilon),$$

based on the definitions in (9).

In the subsequent discussion, we frequently discuss the normal average of a function. We provide its definition and the preliminary properties in the following lemma

LEMMA 4. For a scalar function  $f \in L^2(\Omega_m)$ , we define the normal average  $\bar{f} := \frac{1}{2} \int_{-1}^1 f \, dx_3$ .

(a) The average  $\bar{f}$  is finite for almost all  $y \in U_m$  and  $\|\bar{f}\|_{0,U_m} \leq \frac{1}{\sqrt{2}} \|f\|_{0,\Omega_m}$ .

(b) If  $f \in H^1(\Omega_m)$ , then  $\bar{f} \in H^1(U_m)$ ,  $\partial_\alpha \bar{f} = \overline{\partial_\alpha f}$  and  $\|\bar{f}\|_{1,U_m} \leq \frac{1}{\sqrt{2}} \|f\|_{1,\Omega_m}$ .

(c) If  $f \in H^1(\Omega_m)$ , then  $\overline{x_3 f} = \frac{1}{2} (1 - x_3^2) \partial_3 f$ , a.e.  $U_m$ .

(d) If  $f \in H^1(\tilde{\Omega}^\epsilon)$ , then its normal average on each  $\mathcal{V}_m$  constitutes a global function  $\bar{f} \in H^1(\tilde{\omega})$  and  $\|\bar{f}\|_{H^1(\tilde{\omega})} \leq \frac{C}{\sqrt{\epsilon}} \|f\|_{H^1(\tilde{\Omega}^\epsilon)}$  for some constant  $C > 0$ .

PROOF. See Appendix A.  $\square$

The next lemma, known as *Korn's inequality*, is crucial for deriving our asymptotic result for ADS. This type of inequality was originally established by [Ciarlet et al. 1996], we extend their result to adapt our problem based on a similar proof.

LEMMA 5. (Korn's inequality) For  $\mathbf{v} \in \mathbf{V}_\#(\tilde{\Omega}^\epsilon)$ , we denote its local representation as  $\mathbf{v} = v_{i,m}^\epsilon \mathbf{g}^{i,\epsilon}$  on chart  $(B_m^\epsilon, \Phi_m)$ , the induced strain is given by  $\varepsilon(\mathbf{v}) = e_{i||j,m}^\epsilon(\mathbf{v}) \mathbf{g}^{i,\epsilon} \otimes \mathbf{g}^{j,\epsilon}$ , then for sufficiently small  $\epsilon$ ,

$$\left( \sum_m \sum_i \|v_{i,m}(\epsilon)\|_{1,\mathcal{V}_m}^2 \right)^{1/2} \leq \frac{C}{\epsilon} \left( \sum_m \sum_{i,j} \|e_{i||j,m}(\epsilon)(\mathbf{v})\|_{0,\mathcal{V}_m}^2 \right)^{1/2}.$$

where  $C > 0$  is some constant independent of  $\epsilon$ .<sup>2</sup>

PROOF. See Appendix B.  $\square$

#### 4 Asymptotic directional stiffness

We have defined the *asymptotic directional stiffness* (ADS) in the main text as

$$E_A(\tilde{\omega}) := \lim_{\epsilon \rightarrow 0} \frac{E(\tilde{\Omega}^\epsilon; \epsilon)}{\rho(\tilde{\Omega}^\epsilon)} \quad (30)$$

where  $E(\tilde{\Omega}^\epsilon; \epsilon)$  is given by (3) and  $\rho(\tilde{\Omega}^\epsilon) = |\tilde{\Omega}^\epsilon|/|Y|$  denotes the volume fraction satisfying

$$\rho(\tilde{\Omega}^\epsilon) \sim 2\epsilon |\tilde{\omega}|/|Y| \text{ as } \epsilon \rightarrow 0 \quad (31)$$

For brevity, we introduce the following notation

$$J_\epsilon(\mathbf{u}; \tilde{\omega}; \epsilon) := \frac{1}{2\epsilon |\tilde{\omega}|} \int_{\tilde{\Omega}^\epsilon} (\varepsilon(\mathbf{u}) + \varepsilon) : \mathbf{A} : (\varepsilon(\mathbf{u}) + \varepsilon).$$

We denote

$$J_\epsilon^*(\tilde{\omega}; \epsilon) := \min_{\mathbf{u} \in \mathbf{V}_\#(\tilde{\Omega}^\epsilon)} J_\epsilon(\mathbf{u}; \tilde{\omega}; \epsilon). \quad (32)$$

Then we have

$$E_A(\tilde{\omega}; \epsilon) = \lim_{\epsilon \rightarrow 0} J_\epsilon^*(\tilde{\omega}; \epsilon), \quad (33)$$

according to (3), (30), and (31).

##### 4.1 Convergence theorem

Theorem 1 in the main text is stated as follows:

THEOREM 1. The ADS of  $\tilde{\omega}$  is given by

$$E_A(\tilde{\omega}; \epsilon) = \frac{1}{|\tilde{\omega}|} \int_{\tilde{\omega}} (e_{\tilde{\omega}} + \gamma(\tilde{\mathbf{u}})) : \mathbf{A}_{\tilde{\omega}} : (e_{\tilde{\omega}} + \gamma(\tilde{\mathbf{u}})), \quad (34)$$

where  $\mathbf{A}_{\tilde{\omega}}$  is a fourth-order tensor on  $\tilde{\omega}$  with components

$$a^{\alpha\beta\theta\tau} = \lambda_0 a^{\alpha\beta} a^{\theta\tau} + \mu \left( a^{\alpha\theta} a^{\beta\tau} + a^{\alpha\tau} a^{\beta\theta} \right),$$

<sup>2</sup>In this lemma, we attach the subscript  $m$  of chart to the component of vector and strain tensor for clarity.

and  $\lambda_0 = \frac{2\lambda\mu}{\lambda+2\mu}$ . The notation  $e_{\tilde{\omega}}$  is a second-order tensor signifying the tangent part of  $\varepsilon$  on  $\tilde{\omega}$  with components given by

$$e_{\alpha\beta} = \varepsilon_{ij} \Pi_\alpha^i \Pi_\beta^j.$$

The vector field  $\tilde{\mathbf{u}}$  denotes the solution of the variational equation

$$\int_{\tilde{\omega}} \gamma(\tilde{\mathbf{u}}) : \mathbf{A}_{\tilde{\omega}} : \gamma(\mathbf{v}) = - \int_{\tilde{\omega}} e_{\tilde{\omega}} : \mathbf{A}_{\tilde{\omega}} : \gamma(\mathbf{v}) \text{ for all } \mathbf{v} \in \dot{\mathbf{V}}_\#(\tilde{\omega}), \quad (35)$$

where

$$\gamma_{\alpha\beta}(\boldsymbol{\eta}) := \frac{1}{2} (\partial_\alpha \eta_\beta + \partial_\beta \eta_\alpha) - \Gamma_{\alpha\beta}^\theta \eta_\theta - b_{\alpha\beta} \eta_3 \text{ for } \boldsymbol{\eta} \in H^1(\tilde{\omega})$$

denotes the membrane strain; and the function space is defined as

$$\dot{\mathbf{V}}_\#(\tilde{\omega}) := \text{Completion of } H^1(\tilde{\omega})/\ker \gamma \text{ w.r.t. norm } |\cdot|_{\tilde{\omega}},$$

where norm is given by

$$|\mathbf{v}|_{\tilde{\omega}} := \left( \int_{\tilde{\omega}} \gamma(\mathbf{v}) : \mathbf{A}_{\tilde{\omega}} : \gamma(\mathbf{v}) \right)^{1/2}. \quad (36)$$

REMARK 3. According (34) and (35), the ADS is exactly the minimal value of the following problem

$$E_A(\tilde{\omega}; \epsilon) = \min_{\mathbf{u} \in \dot{\mathbf{V}}_\#(\tilde{\omega})} \frac{1}{|\tilde{\omega}|} \int_{\tilde{\omega}} (e_{\tilde{\omega}} + \gamma(\mathbf{u})) : \mathbf{A}_{\tilde{\omega}} : (e_{\tilde{\omega}} + \gamma(\mathbf{u})). \quad (37)$$

Before the proof of this theorem, we let  $\mathbf{u}^\epsilon$  be the minimizer of (32), namely,

$$\mathbf{u}^\epsilon := \arg \min_{\mathbf{u} \in \mathbf{V}_\#(\tilde{\Omega}^\epsilon)} J_\epsilon(\mathbf{u}; \tilde{\omega}).$$

Note that  $\mathbf{u}^\epsilon$  satisfies the variational equation (2). We define  $u_i(\epsilon)$ ,  $u^j(\epsilon)$  and other geometry symbols on the rescaled parameter domain based on the rules in Section 2.1. For brevity, we denote  $e_{i||j}(\epsilon)(\mathbf{u}^\epsilon)$  as  $e_{i||j}(\epsilon)$ . The proof of Theorem 1 is divided into the following six steps (**Step i~vi**).

**Step i.** On each chart  $(B_m^\epsilon, \Phi_m)$ , the following inequality holds

$$\sum_{i,j} \|e_{i||j}(\epsilon)\|_{0,\mathcal{V}_m} \leq C$$

for some constant  $C > 0$  when  $\epsilon$  is sufficiently small. Consequently, we also have  $\sum_{i,j} \|e_{i||j}(\epsilon)\|_{0,\Omega_m} \leq C$  since  $\Omega_m \subset \mathcal{V}_m$ .

PROOF. This can be deduced from the following inequality

$$\begin{aligned} & \sum_{i,j} \|e_{i||j}(\epsilon)\|_{0,\mathcal{V}_m}^2 \\ & \leq 2 \sum_{i,j} \|e_{i||j}(\epsilon) + g_{ij}(\epsilon)\|_{0,\mathcal{V}_m}^2 + 2 \sum_{i,j} \|g_{ij}(\epsilon)\|_{0,\mathcal{V}_m} \\ & \leq C_2 \int_{\mathcal{V}_m} A^{ijkl}(\epsilon) (e_{i||j}(\epsilon) + g_{ij}(\epsilon)) (e_{k||l}(\epsilon) + g_{kl}(\epsilon)) \sqrt{g(\epsilon)} dx + C_1 \\ & = \frac{C_2}{\epsilon} \int_{B_m^\epsilon} (\varepsilon(\mathbf{u}^\epsilon) + \varepsilon) : \mathbf{A} : (\varepsilon(\mathbf{u}^\epsilon) + \varepsilon) d\tilde{\Omega}^\epsilon + C_1 \\ & \leq C_3 |\tilde{\omega}| J_\epsilon^*(\tilde{\omega}; \epsilon) + C_1 \\ & \leq C_3 |\tilde{\omega}| J_\epsilon(\mathbf{0}; \tilde{\omega}; \epsilon) + C_1 \\ & \leq C_4 |\tilde{\omega}| + C_1, \end{aligned}$$

where  $C_1, C_2, C_3, C_4 > 0$  are some constants independent of  $\epsilon$ . The first inequality holds due to the triangle inequality. The third line is because of the positive definiteness of the elastic tensor (Lemma 3 (29)), the positive lower bound of  $g(\epsilon)$  (Lemma 2 (20)), and the boundness

of the components  $g_{ij}(\epsilon)$  on  $\mathcal{V}_m$ . The fourth and fifth lines follow from the definition of the integral on manifold and the positive integrand. The sixth line holds because  $J_\epsilon^*$  is the minimum of  $J_\epsilon$ . The last inequality results from the direct computation of the constant integral in  $J_\epsilon(\mathbf{0}; \tilde{\omega})$ .  $\square$

**Step ii**. There exists a subsequence of  $\epsilon$  such that on each  $\Omega_m$ ,  $e_{i||j}(\epsilon)$  weakly converges in  $L^2(\Omega_m)$ :

$$e_{i||j}(\epsilon) \rightharpoonup e_{i||j} \quad \text{in } L^2(\Omega_m) \text{ as } \epsilon \rightarrow 0$$

for some  $e_{i||j} \in L^2(\Omega_m)$ .

PROOF. This is the immediate result from the bound in **Step i** on each  $\Omega_m$ , followed by finding the diagonal subsequence of  $\epsilon$  such that the subsequence converges on each  $\Omega_m$  simultaneously. We stress that each  $e_{i||j}$  is only locally defined on one  $\Omega_m$ . We omit the index  $m$  from  $e_{i||j}$  for brevity.  $\square$

REMARK 4. Note the difference:  $e_{\alpha\beta}$  denotes the projection of the macro-strain on surface, while  $e_{\alpha||\beta}$  denotes the weak limit of the strain component induced by the displacement solution  $\mathbf{u}^\epsilon$ .

**Step iii**. For the subsequence we found in **Step ii**, the following weak limit exists on each  $U_m$

$$\left\{ \overline{e_{\alpha||\beta}(\epsilon)} - \gamma_{\alpha\beta}(\overline{\mathbf{u}^\epsilon}) \right\} \rightarrow 0 \quad \text{in } L^2(U_m) \text{ as } \epsilon \rightarrow 0, \quad (38)$$

where ' $\overline{e_{\alpha||\beta}(\epsilon)}$ ' means the normal average on parameter domain defined in Lemma 4; the normal average of the vector field is defined as

$$\overline{\mathbf{u}^\epsilon} := \overline{\hat{u}_i^\epsilon} \mathbf{e}^i,$$

where  $\overline{\hat{u}_i^\epsilon} \in H^1(\tilde{\omega})$  is the globally defined normal average of  $\hat{u}_i^\epsilon \in H^1(\tilde{\Omega}^\epsilon)$  as indicated in Lemma 4(d) and Remark 1.<sup>3</sup> The symbol  $\gamma$  denotes membrane strain, given by

$$\gamma_{\alpha\beta}(\boldsymbol{\eta}) = \frac{1}{2} (\partial_\alpha \eta_\beta + \partial_\beta \eta_\alpha) - \Gamma_{\alpha\beta}^\theta \eta_\theta - b_{\alpha\beta} \eta_3, \quad \text{for } \boldsymbol{\eta} \in \mathbf{H}^1(\tilde{\omega}_m).$$

Here, the function space  $\mathbf{H}^1(\tilde{\omega}_m) := \{ \hat{\eta}_i \mathbf{e}^i : \hat{\eta}_i \in H^1(\tilde{\omega}_m) \}$ .

PROOF. We prove the following two limits that yield the conclusion:

$$\left\{ \overline{e_{\alpha||\beta}(\epsilon)} - \gamma_{\alpha\beta}(\overline{\mathbf{u}^\epsilon} \mathbf{a}^i) \right\} \rightarrow 0 \quad \text{in } L^2(U_m) \text{ as } \epsilon \rightarrow 0, \quad (39)$$

$$\left\{ \gamma_{\alpha\beta}(\overline{\mathbf{u}^\epsilon} \mathbf{a}^i) - \gamma_{\alpha\beta}(\overline{\hat{u}_i^\epsilon} \mathbf{e}^i) \right\} \rightarrow 0 \quad \text{in } L^2(U_m) \text{ as } \epsilon \rightarrow 0, \quad (40)$$

First, we show that  $\overline{\mathbf{u}^\epsilon} \mathbf{a}^i, \overline{\hat{u}_i^\epsilon} \mathbf{e}^i \in \mathbf{H}^1(\tilde{\omega}_m)$ . Consider the following identities

$$\begin{aligned} \overline{\mathbf{u}^\epsilon} \mathbf{a}^i &= \overline{u_j^\epsilon \Xi_i^j} \mathbf{e}^i, \\ \overline{\hat{u}_i^\epsilon} \mathbf{e}^i &= \overline{u_k^\epsilon \Pi_i^{k,\epsilon}} \mathbf{e}^i. \end{aligned}$$

We note  $\Xi_i^j \in C^\infty(\mathcal{U}_m)$ ,  $\Pi_i^{k,\epsilon} \in C^\infty(\mathcal{V}_m^\epsilon)$  and they are continuous to the boundary of  $\mathcal{U}_m$  and  $\mathcal{V}_m^\epsilon$ , respectively (see Remark 1). Additionally, we know  $u_i^\epsilon \in H^1(\Omega_m^\epsilon)$ . Then we can deduce  $\overline{u_j^\epsilon \Xi_i^j}, \overline{u_k^\epsilon \Pi_i^{k,\epsilon}} \in H^1(\tilde{\omega}_m)$  according to Lemma 4. Therefore, both vector fields are in  $\mathbf{H}^1(\tilde{\omega}_m)$ .

<sup>3</sup>Recall that  $\hat{u}_i^\epsilon$  is the covariant component of vector field  $\mathbf{u}^\epsilon$  under canonical basis  $\{\mathbf{e}^i\}$ , and  $u_i^\epsilon$  is the covariant component under local basis  $\{\mathbf{g}^{i,\epsilon}\}$ .

Next, we apply Lemma 4(b) and get

$$\begin{aligned} & \overline{e_{\alpha||\beta}(\epsilon)} - \gamma_{\alpha\beta}(\overline{\mathbf{u}^\epsilon} \mathbf{a}^i) \\ &= \frac{1}{2} (\partial_\alpha u_\beta(\epsilon) + \partial_\beta u_\alpha(\epsilon)) - \Gamma_{\alpha\beta}^\sigma(\epsilon) u_\sigma(\epsilon) - \Gamma_{\alpha\beta}^3(\epsilon) u_3(\epsilon) \\ & \quad - \frac{1}{2} (\partial_\alpha \overline{u_\beta(\epsilon)} + \partial_\beta \overline{u_\alpha(\epsilon)}) + \Gamma_{\alpha\beta}^\sigma \overline{u_\sigma(\epsilon)} + b_{\alpha\beta} \overline{u_3(\epsilon)} \\ &= \overline{\Gamma_{\alpha\beta}^{\sigma,2}(\epsilon) u_\sigma(\epsilon)} + \overline{\epsilon x_3 b_\beta^\sigma |_\alpha u_\sigma(\epsilon)} + \overline{\epsilon x_3 c_{\alpha\beta} u_3(\epsilon)}, \end{aligned} \quad (41)$$

where

$$\Gamma_{\alpha\beta}^{\sigma,2}(\epsilon) := \left\{ \Gamma_{\alpha\beta}^\sigma - \epsilon x_3 b_\beta^\sigma |_\alpha \right\} - \Gamma_{\alpha\beta}^\sigma(\epsilon)$$

satisfies

$$\left\| \Gamma_{\alpha\beta}^{\sigma,2}(\epsilon) \right\|_{0,\infty,\Omega_m} \lesssim \epsilon^2 \quad (42)$$

according to Lemma 3 (27). Applying Lemma 4 (a) and (c) yields

$$\begin{aligned} \|\overline{x_3 v}\|_{0,U_m} &= \left\| \frac{1}{2} (1 - x_3^2) \partial_3 v \right\|_{0,U_m} \\ &\lesssim \frac{1}{2} (1 - x_3^2) \partial_3 v \|_{0,\Omega_m} \lesssim \|\partial_3 v\|_{0,\Omega_m}, \quad \forall v \in H^1(\Omega_m), \end{aligned}$$

where the last inequality holds because  $|\frac{1}{2}(1 - x_3^2)| \leq 1$ . Therefore,

$$\begin{aligned} \|\overline{x_3 b_\beta^\sigma |_\alpha u_\sigma(\epsilon)}\|_{0,U_m} &\lesssim \sum_\sigma \|\partial_3 (b_\beta^\sigma |_\alpha u_\sigma(\epsilon))\|_{0,\Omega_m} \lesssim \|\partial_3 u_\sigma(\epsilon)\|_{0,\Omega_m} \\ \|\overline{x_3 c_{\alpha\beta} u_3(\epsilon)}\|_{0,U_m} &\lesssim \|\partial_3 (c_{\alpha\beta} u_3(\epsilon))\|_{0,\Omega_m} \lesssim \|\partial_3 u_3(\epsilon)\|_{0,\Omega_m}, \end{aligned} \quad (43)$$

where we have used the condition that  $b_\beta^\sigma |_\alpha$  and  $c_{\alpha\beta}$  are independent of  $x_3$ , and both are bounded in  $U_m$ . Consequently, it follows from (41), (42) and (43) that

$$\begin{aligned} & \left\| \overline{e_{\alpha||\beta}(\epsilon)} - \gamma_{\alpha\beta}(\overline{\mathbf{u}^\epsilon} \mathbf{g}^i) \right\|_{0,U_m} \\ & \lesssim \epsilon \left\{ \sum_\alpha \|\epsilon u_\alpha(\epsilon)\|_{0,\Omega_m} + \sum_i \|\partial_3 u_i(\epsilon)\|_{0,\Omega_m} \right\}. \end{aligned} \quad (44)$$

From Korn's inequality (Lemma 5), we know

$$\|\epsilon u_\alpha(\epsilon)\|_{0,\Omega_m} \leq \epsilon \|u_\alpha(\epsilon)\|_{1,\Omega_m} \lesssim \left\{ \sum_m \sum_{i,j} \|e_{i||j}(\epsilon)\|_{0,\mathcal{V}_m}^2 \right\}^{1/2}, \quad (45)$$

where the last term has a constant upper bound from **Step i**.

Then according to the definition of  $e_{i||j}(\epsilon)$ , the following equalities hold

$$\begin{aligned} \partial_3 u_\alpha(\epsilon) &= 2\epsilon e_{\alpha||3}(\epsilon) - \epsilon \partial_\alpha u_3(\epsilon) + 2\epsilon \Gamma_{\alpha 3}^\sigma(\epsilon) u_\sigma(\epsilon), \\ \partial_3 u_3(\epsilon) &= \epsilon e_{3||3}(\epsilon). \end{aligned}$$

Thus, we have the relation

$$\begin{aligned} \sum_i \|\partial_3 u_i(\epsilon)\|_{0,\Omega_m} &\lesssim \epsilon \left( \sum_{i,j} \|e_{i||j}(\epsilon)\|_{0,\Omega_m} + \sum_i \|u_i(\epsilon)\|_{1,\Omega_m} \right) \\ &\lesssim \left\{ \sum_m \sum_{i,j} \|e_{i||j}(\epsilon)\|_{0,\Omega_m}^2 \right\}^{1/2}. \end{aligned} \quad (46)$$

Again, from the upper bound in **Step i**, the last term is bounded. Hence, the right hand side of (44) tends to 0 as  $\epsilon \rightarrow 0$  from (45) and (46). Then (39) is proved from (44).

Next, we let

$$\mathbf{w}^\epsilon := \overline{\hat{u}_i^\epsilon} \mathbf{e}^i.$$

Through integration by parts, the following relation holds for any  $\phi \in \mathcal{D}(U_m)$ :

$$\begin{aligned} & \left| \int_{U_m} \left( \gamma_{\alpha\beta}(\bar{u}_i^\epsilon \mathbf{g}^i) - \gamma_{\alpha\beta}(\mathbf{w}^\epsilon) \right) \phi \, ds \right| \\ & \lesssim \|\bar{u}_\beta(\epsilon) - w_\beta^\epsilon\|_{0,U_m} \|\partial_\alpha \phi\|_{0,U_m} + \|\bar{u}_\alpha(\epsilon) - w_\alpha^\epsilon\|_{0,U_m} \|\partial_\beta \phi\|_{0,U_m} \\ & \quad + \|\bar{u}_\sigma(\epsilon) - w_\sigma^\epsilon\|_{0,U_m} \|\phi\|_{0,U_m} + \|\bar{u}_3(\epsilon) - w_3^\epsilon\|_{0,U_m} \|\phi\|_{0,U_m}. \end{aligned} \quad (47)$$

Here, we have used Cauchy's inequality and the boundness of  $\Gamma_{\alpha\beta}^\sigma, b_{\alpha\beta}$  in the second inequality. Note that

$$\overline{u_i(\epsilon)} - w_i^\epsilon = \overline{u_i(\epsilon)} - \overline{\hat{u}_k(\epsilon)} \Pi_i^k = \overline{(\delta_i^j - \Pi_i^k \Xi_k^j(\epsilon)) u_j(\epsilon)},$$

From Lemma 2, we can see that

$$\begin{aligned} \Pi_\alpha^k \Xi_k^\sigma(\epsilon) &= \Pi_\alpha^k(\Xi_k^\sigma + \epsilon x_3 b_\theta^\sigma \Xi_k^\theta + R_\theta^\sigma(\epsilon) \Xi_k^\theta) = \delta_\alpha^\sigma + \epsilon x_3 b_\alpha^\sigma + R_\alpha^\sigma(\epsilon) \\ \Pi_3 \Xi_k^3(\epsilon) &= \Pi_\alpha^k \Xi_k^3(\epsilon) = 0 \\ \Pi_3^k \Xi_k^3(\epsilon) &= 1. \end{aligned}$$

Therefore, we obtain the following two relations:

$$\begin{aligned} \overline{u_\alpha(\epsilon)} - w_\alpha^\epsilon &= \overline{(\delta_\alpha^j - \Pi_\alpha^k \Xi_k^j(\epsilon)) u_j(\epsilon)} = \overline{\{\epsilon x_3 b_\alpha^\sigma + R_\alpha^\sigma(\epsilon)\} u_\sigma(\epsilon)} \\ \overline{u_3(\epsilon)} - w_3^\epsilon &= \overline{(\delta_3^j - \Pi_3^k \Xi_k^j(\epsilon)) u_j(\epsilon)} = 0 \end{aligned}$$

Then, the following equality holds:

$$\overline{u_\alpha(\epsilon)} - w_\alpha^\epsilon - \overline{\epsilon x_3 b_\alpha^\sigma u_\sigma(\epsilon)} = \overline{R_\alpha^\sigma(\epsilon) u_\sigma(\epsilon)}. \quad (48)$$

According to Lemma 4(b) and Lemma 2 (26), we know

$$\|\overline{R_\alpha^\sigma(\epsilon) u_\sigma(\epsilon)}\|_{1,U_m} \lesssim \epsilon \sum_j \|\overline{\epsilon u_j(\epsilon)}\|_{1,U_m} \lesssim \epsilon \left( \sum_j \|\epsilon u_j(\epsilon)\|_{1,\Omega_m}^2 \right)^{1/2} \quad (49)$$

$$\|\overline{\epsilon x_3 b_\alpha^\sigma u_\sigma(\epsilon)}\|_{1,U_m} \lesssim \|\epsilon x_3 b_\alpha^\sigma u_\sigma(\epsilon)\|_{1,\Omega_m}. \quad (50)$$

From the upper bound in **Step i** and Korn's inequality (Lemma 5), the last term of (49) vanishes as  $\epsilon \rightarrow 0$  and the last term of (50) is bounded. On the other hand, we leverage Lemma 4 (a)(c), (49), and (46) and deduce the following relation

$$\begin{aligned} \|\overline{\epsilon x_3 b_\alpha^\sigma u_\sigma(\epsilon)}\|_{0,U_m} &= \epsilon \left\| \frac{1}{2} (1 - x_3^2) b_\alpha^\sigma \partial_3 u_\sigma(\epsilon) \right\|_{0,U_m} \\ &\lesssim \epsilon \sum_\sigma \|\overline{\partial_3 u_\sigma(\epsilon)}\|_{0,U_m} \lesssim \epsilon \sum_\sigma \|\partial_3 u_\sigma(\epsilon)\|_{0,\Omega_m} \rightarrow 0. \end{aligned} \quad (51)$$

The first equality is based on the fact that  $b_\alpha^\sigma$  is independent of  $x_3$ . Combining (48), (49), (50), and (51) leads to the following conclusions

- $\|\bar{u}_\alpha(\epsilon) - w_\alpha^\epsilon\|_{1,U_m}$  is bounded as  $\epsilon \rightarrow 0$ .
- $\|\bar{u}_\alpha(\epsilon) - w_\alpha^\epsilon\|_{0,U_m} \rightarrow 0$  as  $\epsilon \rightarrow 0$ .

Hence, we use (47) to get the following limit

$$\int_{U_m} \left( \gamma_{\alpha\beta}(\bar{u}_i^\epsilon \mathbf{g}^i) - \gamma_{\alpha\beta}(\mathbf{w}^\epsilon) \right) \phi \, ds \rightarrow 0, \quad \forall \phi \in \mathcal{D}(U_m)$$

Since  $\mathcal{D}(U_m)$  is dense in  $L^2(U_m)$ , to justify the weak convergence (40), it suffices to show that  $\gamma_{\alpha\beta}(\bar{u}_i^\epsilon \mathbf{g}^i) - \gamma_{\alpha\beta}(\mathbf{w}^\epsilon)$  is bounded in  $L^2(U_m)$  independent of  $\epsilon$ . This can be immediately deduced from the boundness of  $\|\bar{u}_i(\epsilon) - w_i^\epsilon\|_{1,U_m}$  and the relation

$$\|\gamma_{\alpha\beta}(\bar{u}_i^\epsilon \mathbf{g}^i) - \gamma_{\alpha\beta}(\mathbf{w}^\epsilon)\|_{0,U_m} \lesssim \sum_i \|\bar{u}_i(\epsilon) - w_i^\epsilon\|_{1,U_m},$$

which is derived by definition of  $\gamma$ . □

**Step iv.** The space  $\dot{V}_\#(\tilde{\omega})$  is a Hilbert space, and there exist  $\bar{\mathbf{u}} \in \dot{V}_\#(\tilde{\omega})$  and a subsequence of the subsequence we found in **Step ii** such that

$$\bar{\mathbf{u}}^\epsilon \rightharpoonup \bar{\mathbf{u}} \quad \text{in } \dot{V}_\#(\tilde{\omega}). \quad (52)$$

Furthermore, the limit  $\bar{\mathbf{u}}$  is the unique solution of the variational equation (35).

**PROOF.** Since  $\mathbf{A}_{\tilde{\omega}}$  is a positive definite tensor, the following bilinear form defines an inner product on  $\mathbf{H}^1(\tilde{\omega})/\ker \gamma$ :

$$\langle \boldsymbol{\eta}, \boldsymbol{\xi} \rangle := \int_{\tilde{\omega}} \gamma(\boldsymbol{\eta}) : \mathbf{A}_{\tilde{\omega}} : \gamma(\boldsymbol{\xi}).$$

The norm defined in (36) is exactly induced by this inner product. Therefore, the space  $\dot{V}_\#(\tilde{\omega})$  is a Hilbert space.

To show that there exist a subsequence that weakly converges, we only need to show  $|\bar{\mathbf{u}}^\epsilon|_{\tilde{\omega}}$  is bounded independent of  $\epsilon$ . According to (38), we know  $\|e_{\alpha\|\beta}(\epsilon) - \gamma_{\alpha\beta}(\bar{\mathbf{u}}^\epsilon)\|_{0,U_m}$  is bounded independent of  $\epsilon$  on each  $U_m$ . We also have  $\|e_{\alpha\|\beta}(\epsilon)\|_{0,U_m} \leq \frac{1}{\sqrt{2}} \|e_{\alpha\|\beta}(\epsilon)\|_{0,\Omega_m}$  from Lemma 4b that implies  $\|e_{\alpha\|\beta}(\epsilon)\|_{0,U_m}$  bounded from **Step i**. Hence, we know  $\gamma_{\alpha\beta}(\bar{\mathbf{u}}^\epsilon)$  is bounded independent of  $\epsilon$  in  $L^2(U_m)$ . Given that

$$|\bar{\mathbf{u}}^\epsilon|_{\tilde{\omega}}^2 = \int_{\tilde{\omega}} \gamma(\bar{\mathbf{u}}^\epsilon) : \mathbf{A}_{\tilde{\omega}} : \gamma(\bar{\mathbf{u}}^\epsilon) \lesssim \int_{\tilde{\omega}} \|\gamma(\bar{\mathbf{u}}^\epsilon)\|^2$$

we know  $|\bar{\mathbf{u}}^\epsilon|_{\tilde{\omega}}$  is bounded. Therefore, such weakly converged subsequence exist and we still denote it as  $\bar{\mathbf{u}}^\epsilon$  for brevity.

We then show that this subsequence converges in  $\dot{V}_\#(\tilde{\omega})$  to some  $\bar{\mathbf{u}} \in \dot{V}_\#(\tilde{\omega})$  and it satisfies (35). Suppose  $\mathbf{v} \in \mathbf{H}^1(\tilde{\omega})/\ker \gamma$ , we identify it as a function defined on  $\tilde{\Omega}^\epsilon$  that is constant along normal direction. Then, we substitute it into the weak form equation and obtain

$$\int_{\tilde{\Omega}^\epsilon} \boldsymbol{\varepsilon}(\mathbf{u}^\epsilon) : \mathbf{A} : \boldsymbol{\varepsilon}(\mathbf{v}) = - \int_{\tilde{\Omega}^\epsilon} \boldsymbol{\varepsilon} : \mathbf{A} : \boldsymbol{\varepsilon}(\mathbf{v})$$

Split the integral onto charts, we get

$$\begin{aligned} & \sum_m \int_{\Omega_m} A^{ijkl}(\epsilon) e_{i\|j}(\epsilon) e_{k\|l}(\epsilon)(\mathbf{v}) \sqrt{g(\epsilon)} \\ &= - \sum_m \int_{\Omega_m} A^{ijkl}(\epsilon) e_{ij}(\epsilon) e_{k\|l}(\epsilon)(\mathbf{v}) \sqrt{g(\epsilon)}. \end{aligned} \quad (53)$$

As  $\mathbf{v}$  is constant w.r.t.  $x_3$ , we can verify based on Lemma 3 and Remark 2 that

$$\begin{aligned} e_{\alpha\|\beta}(\epsilon)(\mathbf{v}) &\rightarrow \gamma_{\alpha\beta}(\mathbf{v}) \quad \text{in } L^2(\Omega_m), \\ e_{\alpha\|3}(\epsilon)(\mathbf{v}) &\rightarrow \left\{ \frac{1}{2} \partial_\alpha v_3 + b_\alpha^\sigma v_\sigma \right\} \quad \text{in } L^2(\Omega_m), \\ e_{3\|3}(\epsilon)(\mathbf{v}) &= 0. \end{aligned}$$

Then, the LHS of (53) converges to the following limit

$$\begin{aligned}
& \int_{\Omega_m} A^{ijkl}(\epsilon) e_{i||j}(\epsilon) e_{k||l}(\epsilon) (v) \sqrt{g(\epsilon)} \\
& \rightarrow \int_{\Omega_m} \left( A^{\alpha\beta\theta\tau}(0) e_{\theta||\tau} + A^{\alpha\beta 33}(0) e_{3||3} \right) \gamma_{\alpha\beta}(v) \sqrt{a} \, dx \\
& + \int_{\Omega_m} 4A^{\alpha 3\sigma 3}(0) e_{\sigma||3} \left\{ \frac{1}{2} \partial_\alpha v_3 + b_\alpha^\sigma v_\sigma \right\} \sqrt{a} \, dx \\
& = \int_{\Omega_m} \left\{ a^{\alpha\beta\theta\tau} e_{\theta||\tau} \gamma_{\alpha\beta}(v) \right. \\
& - \frac{\lambda}{\lambda + 2\mu} a^{\alpha\beta} \left( (\lambda + 2\mu) e_{33} + \lambda a^{\theta\tau} e_{\theta\tau} \right) \gamma_{\alpha\beta}(v) \left. \right\} \sqrt{a} \, dx \\
& - \int_{\Omega_m} 4\mu a^{\alpha\sigma} e_{\sigma 3} \left\{ \frac{1}{2} \partial_\alpha v_3 + b_\alpha^\sigma v_\sigma \right\} \sqrt{a} \, dx
\end{aligned} \tag{54}$$

and the RHS of (53) converges to another limit

$$\begin{aligned}
& \int_{\Omega_m} A^{ijkl}(\epsilon) e_{ij}(\epsilon) e_{kl}(\epsilon) (v) \sqrt{g(\epsilon)} \\
& \rightarrow \int_{\Omega_m} \left( A^{\alpha\beta\theta\tau}(0) e_{\theta\tau} + A^{\alpha\beta 33}(0) e_{33} \right) \gamma_{\alpha\beta}(v) \sqrt{a} \, dx \\
& + \int_{\Omega_m} 4A^{\alpha 3\sigma 3}(0) e_{\sigma 3} \left\{ \frac{1}{2} \partial_\alpha v_3 + b_\alpha^\sigma v_\sigma \right\} \sqrt{a} \, dx \\
& = \int_{\Omega_m} \left\{ \lambda a^{\alpha\beta} a^{\theta\tau} e_{\theta\tau} + 2\mu a^{\alpha\theta} a^{\beta\tau} e_{\theta\tau} + \lambda a^{\alpha\beta} e_{33} \right\} \gamma_{\alpha\beta}(v) \sqrt{a} \, dx \\
& + \int_{\Omega_m} 4\mu a^{\alpha\sigma} e_{\sigma 3} \left\{ \frac{1}{2} \partial_\alpha v_3 + b_\alpha^\sigma v_\sigma \right\} \sqrt{a} \, dx.
\end{aligned} \tag{55}$$

Combining the limits in (54) and (55) and eliminate the same terms, we can deduce that

$$\sum_m \int_{\Omega_m} a^{\alpha\beta\theta\tau} e_{\theta||\tau} \gamma_{\alpha\beta}(v) \sqrt{a} \, dx = - \sum_m \int_{\Omega_m} a^{\alpha\beta\theta\tau} e_{\theta\tau} \gamma_{\alpha\beta}(v) \sqrt{a} \, dx. \tag{56}$$

It follows from (38) that

$$\begin{aligned}
& \sum_m \int_{\Omega_m} a^{\alpha\beta\theta\tau} e_{\theta||\tau} \gamma_{\alpha\beta}(v) \sqrt{a} \, dx \\
& = \lim_{\epsilon \rightarrow 0} \sum_m \int_{\Omega_m} a^{\alpha\beta\theta\tau} e_{\theta||\tau}(\epsilon) \gamma_{\alpha\beta}(v) \sqrt{a} \, dx \\
& = \lim_{\epsilon \rightarrow 0} \sum_m \int_{U_m} a^{\alpha\beta\theta\tau} \overline{e_{\theta||\tau}(\epsilon)} \gamma_{\alpha\beta}(v) \sqrt{a} \, dx \\
& = \lim_{\epsilon \rightarrow 0} \sum_m \int_{U_m} a^{\alpha\beta\theta\tau} \gamma_{\theta\tau}(\overline{u^\epsilon}) \gamma_{\alpha\beta}(v) \sqrt{a} \, dx \\
& = \sum_m \int_{U_m} a^{\alpha\beta\theta\tau} \gamma_{\theta\tau}(\overline{u}) \gamma_{\alpha\beta}(v) \sqrt{a} \, dx,
\end{aligned} \tag{57}$$

where the last equality has utilized the condition (52), namely,

$$\langle \overline{u^\epsilon}, v \rangle \rightarrow \langle \overline{u}, v \rangle, \quad \text{as } \epsilon \rightarrow 0.$$

From (56) and (57), we arrive at the equation

$$\int_{\tilde{\omega}} \gamma(\overline{u}) : A_{\tilde{\omega}} : \gamma(v) = - \int_{\tilde{\omega}} e_{\tilde{\omega}} : A_{\tilde{\omega}} : \gamma(v), \quad \forall v \in H^1(\tilde{\omega})/\ker \gamma. \tag{58}$$

Now, we suppose  $v \in \dot{V}_\#(\tilde{\omega})$  (which may not be in  $H^1(\tilde{\omega})/\ker \gamma$ ), we let

$$\begin{aligned}
\dot{B}(\eta, \xi) &:= \int_{\tilde{\omega}} \gamma(\eta) : A_{\tilde{\omega}} : \gamma(\xi) \\
\dot{L}(\xi) &:= - \int_{\tilde{\omega}} e_{\tilde{\omega}} : A_{\tilde{\omega}} : \gamma(\xi).
\end{aligned}$$

As  $A_{\tilde{\omega}}$  is positive definite, we have

$$|\dot{L}(\xi)|^2 \leq \int_{\tilde{\omega}} \|A_{\tilde{\omega}} : e_{\tilde{\omega}}\|^2 \int_{\tilde{\omega}} \|\gamma(\xi)\|^2 \lesssim |\xi|_{\tilde{\omega}}^2, \quad \forall \xi \in H^1(\tilde{\omega}),$$

where the second inequality is due to the positive definiteness of  $A_{\tilde{\omega}}$ . Thus, it shows that  $\dot{L}$  is continuous. The bilinear form  $\dot{B}$  is also continuous as it is exactly the inner product in  $\dot{V}_\#(\tilde{\omega})$ . Therefore, we can find a sequence  $v^n \in H^1(\tilde{\omega})/\ker \gamma$  that approaches  $v$  in  $\dot{V}_\#(\tilde{\omega})$  and each  $v^n$  satisfies (58). By letting  $n \rightarrow \infty$ , (58) still holds for  $v$  due to continuity of  $\dot{B}$  and  $\dot{L}$ . Therefore, (35) is proved for any  $v \in \dot{V}_\#(\tilde{\omega})$ . As  $\dot{B}, \dot{L}$  are continuous and  $\dot{B}$  is elliptic, we know (35) has unique solution by Lax–Milgram theorem.  $\square$

**Step v.** For the subsequence we found in **Step vi**, we have the following limit

$$\lim_{\epsilon \rightarrow 0} J_\epsilon^*(\tilde{\omega}; \epsilon) = \frac{1}{|\tilde{\omega}|} \int_{\tilde{\omega}} (\gamma(\overline{u}) + e_{\tilde{\omega}}) : A_{\tilde{\omega}} : (\gamma(\overline{u}) + e_{\tilde{\omega}}). \tag{59}$$

PROOF. Split the integral of  $J_\epsilon^*(\tilde{\omega})$  onto charts:

$$\begin{aligned}
J_\epsilon^*(\tilde{\omega}; \epsilon) &= \frac{1}{2\epsilon|\tilde{\omega}|} \int_{\tilde{\Omega}^\epsilon} (\epsilon(u^\epsilon) + \epsilon) : A : (\epsilon(u^\epsilon) + \epsilon) \, d\tilde{\Omega}^\epsilon \\
&= \frac{1}{2\epsilon|\tilde{\omega}|} \int_{\tilde{\Omega}^\epsilon} \epsilon(u^\epsilon) : A : \epsilon d\tilde{\Omega}^\epsilon + \frac{1}{2\epsilon|\tilde{\omega}|} \int_{\tilde{\Omega}^\epsilon} \epsilon : A : \epsilon d\tilde{\Omega}^\epsilon \\
&= \frac{1}{2\epsilon|\tilde{\omega}|} \int_{\tilde{\Omega}^\epsilon} \epsilon : A : \epsilon d\tilde{\Omega}^\epsilon \\
&+ \sum_m \frac{1}{2|\tilde{\omega}|} \int_{\Omega_m} A^{ijkl}(\epsilon) e_{i||j}(\epsilon) e_{k||l}(\epsilon) \sqrt{g(\epsilon)} \, dx.
\end{aligned} \tag{60}$$

where

$$e_{ij}(\epsilon) = \epsilon_{kl} \Pi_i^k(\epsilon) \Pi_j^l(\epsilon)$$

denotes the components of macro-strain under local coordinate system.

Due to the constant integrand, the first integral in (60) tends to the following limit as  $\epsilon \rightarrow 0$ :

$$\frac{1}{2\epsilon|\tilde{\omega}|} \int_{\tilde{\Omega}^\epsilon} \epsilon : A : \epsilon d\tilde{\Omega}^\epsilon \rightarrow T(\epsilon),$$

where

$$T(\epsilon) := \lambda |\text{tr } \epsilon|^2 + 2\mu \|\epsilon\|_F^2. \tag{61}$$

For the last integral, we have the following limit as  $\epsilon \rightarrow 0$

$$\begin{aligned}
 & \frac{1}{2|\tilde{\omega}|} \int_{\Omega_m} A^{ijkl}(\epsilon) e_{i||j}(\epsilon) e_{kl}(\epsilon) \sqrt{g(\epsilon)} dx \\
 &= \frac{1}{2|\tilde{\omega}|} \left\{ \int_{\Omega_m} \left( A^{\alpha\beta\theta\tau}(\epsilon) e_{\theta\tau}(\epsilon) + A^{\alpha\beta 33}(\epsilon) e_{33}(\epsilon) \right) e_{\alpha||\beta}(\epsilon) \sqrt{g(\epsilon)} dx \right. \\
 &+ \int_{\Omega_m} 4A^{\alpha 3\sigma 3}(\epsilon) e_{\sigma 3}(\epsilon) e_{\alpha||3}(\epsilon) \sqrt{g(\epsilon)} dx \\
 &+ \left. \int_{\Omega_m} \left( A^{33\theta\tau}(\epsilon) e_{\theta\tau}(\epsilon) + A^{3333}(\epsilon) e_{33}(\epsilon) \right) e_{3||3}(\epsilon) \sqrt{g(\epsilon)} dx \right\} \\
 &\rightarrow \frac{1}{2|\tilde{\omega}|} \left\{ \int_{\Omega_m} \left( A^{\alpha\beta\theta\tau}(0) e_{\theta\tau} + A^{\alpha\beta 33}(0) e_{33} \right) e_{\alpha||\beta} \sqrt{a} dx \right. \\
 &+ \int_{\Omega_m} 4A^{\alpha 3\sigma 3}(0) e_{\sigma 3} e_{\alpha||3} \sqrt{a} dx \\
 &+ \left. \int_{\Omega_m} \left( A^{33\theta\tau}(0) e_{\theta\tau} + A^{3333}(0) e_{33} \right) e_{3||3} \sqrt{a} dx \right\} \\
 &= \frac{1}{2|\tilde{\omega}|} \int_{\Omega_m} a^{\alpha\beta\theta\tau} e_{\theta\tau} e_{\alpha||\beta} \sqrt{a} dx - S_m,
 \end{aligned}$$

where

$$a^{\alpha\beta\theta\tau} = \lambda_0 a^{\alpha\beta} a^{\theta\tau} + \mu \left( a^{\alpha\theta} a^{\beta\tau} + a^{\alpha\tau} a^{\beta\theta} \right)$$

and  $\lambda_0 = \frac{2\lambda\mu}{\lambda+2\mu}$ . The constant term  $S_m$  is computed as

$$\begin{aligned}
 S_m := \frac{1}{|\tilde{\omega}|} \int_{U_m} & \left( \frac{\lambda^2}{\lambda+2\mu} a^{\alpha\beta} a^{\theta\tau} e_{\alpha\beta} e_{\theta\tau} + 2\lambda a^{\alpha\beta} e_{33} e_{\alpha\beta} \right. \\
 & \left. + (\lambda+2\mu) e_{33} e_{33} + 2\mu a^{\alpha\beta} e_{\alpha 3} e_{\beta 3} \right) \sqrt{a}.
 \end{aligned} \quad (62)$$

We define

$$E_M := T(\epsilon) - \sum_m S_m(\epsilon).$$

According to (61) and (62), we have

$$E_M = \frac{1}{|\tilde{\omega}|} \sum_m \int_{U_m} a^{\alpha\beta\theta\tau} e_{\alpha\beta} e_{\theta\tau} \sqrt{a},$$

which can also be written in matrix form as

$$E_M = \int_{\tilde{\omega}} \lambda_0 \left( \text{tr } P^\top \epsilon P \right)^2 + 2\mu \|P^\top \epsilon P\|_F^2,$$

where  $P := \mathbf{I} - \mathbf{nn}^\top$  is the projection matrix to the tangent space of  $\tilde{\omega}$ .

In summary, we have

$$J_\epsilon^*(\tilde{\omega}) \rightarrow E_M + \sum_m \frac{1}{2|\tilde{\omega}|} \int_{\Omega_m} a^{\alpha\beta\theta\tau} e_{\alpha\beta} e_{\theta\tau} \sqrt{a} dx. \quad (63)$$

Note that the summand of the last term in (63) can be expressed as an integral on the mid-surface

$$\frac{1}{2|\tilde{\omega}|} \int_{\Omega_m} a^{\alpha\beta\theta\tau} e_{\alpha\beta} e_{\theta\tau} \sqrt{a} dx = \frac{1}{|\tilde{\omega}|} \int_{U_m} a^{\alpha\beta\theta\tau} e_{\alpha\beta} \overline{e_{\theta\tau}} \sqrt{a} ds.$$

Since  $e_{\theta||\tau}(\epsilon) \rightharpoonup e_{\theta||\tau}$  in  $L^2(\Omega_m)$  by **Step ii**, we have

$$\begin{aligned}
 \frac{1}{|\tilde{\omega}|} \int_{U_m} a^{\alpha\beta\theta\tau} e_{\alpha\beta} \overline{e_{\theta||\tau}(\epsilon)} \sqrt{a} ds &= \frac{1}{2|\tilde{\omega}|} \int_{\Omega_m} a^{\alpha\beta\theta\tau} e_{\alpha\beta} e_{\theta||\tau}(\epsilon) \sqrt{a} dx \\
 &\rightarrow \frac{1}{2|\tilde{\omega}|} \int_{\Omega_m} a^{\alpha\beta\theta\tau} e_{\alpha\beta} e_{\theta||\tau} \sqrt{a} dx.
 \end{aligned} \quad (64)$$

We apply **Step iii** (38) in (64), which gives the following limit

$$\frac{1}{|\tilde{\omega}|} \int_{U_m} a^{\alpha\beta\theta\tau} e_{\alpha\beta} \gamma_{\theta\tau}(\bar{\mathbf{u}}^\epsilon) \sqrt{a} ds \rightarrow \frac{1}{2|\tilde{\omega}|} \int_{\Omega_m} a^{\alpha\beta\theta\tau} e_{\alpha\beta} e_{\theta||\tau} \sqrt{a} dx. \quad (65)$$

According to **Step iv** (52) and the continuity of  $\dot{L}$ , we also have

$$\sum_m \int_{U_m} a^{\alpha\beta\theta\tau} e_{\alpha\beta} \gamma_{\theta\tau}(\bar{\mathbf{u}}^\epsilon) \sqrt{a} ds = -\dot{L}(\bar{\mathbf{u}}^\epsilon) \rightarrow -\dot{L}(\bar{\mathbf{u}}). \quad (66)$$

Based on (65) and (66), we obtain

$$\begin{aligned}
 \sum_m \frac{1}{2|\tilde{\omega}|} \int_{\Omega_m} a^{\alpha\beta\theta\tau} e_{\alpha\beta} e_{\theta||\tau} \sqrt{a} dx &= -\frac{1}{|\tilde{\omega}|} \dot{L}(\bar{\mathbf{u}}) \\
 &= \frac{1}{|\tilde{\omega}|} \int_{\tilde{\omega}} e_{\tilde{\omega}} : \mathbf{A}_{\tilde{\omega}} : \gamma(\bar{\mathbf{u}}).
 \end{aligned}$$

Finally, we substitute above equation into (63) and get the following limit

$$\begin{aligned}
 J_\epsilon^*(\epsilon) &\rightarrow E_M + \frac{1}{|\tilde{\omega}|} \int_{\tilde{\omega}} e_{\tilde{\omega}} : \mathbf{A}_{\tilde{\omega}} : \gamma(\bar{\mathbf{u}}) \\
 &= \frac{1}{|\tilde{\omega}|} \int_{\tilde{\omega}} (\gamma(\bar{\mathbf{u}}) + e_{\tilde{\omega}}) : \mathbf{A}_{\tilde{\omega}} : e_{\tilde{\omega}} \\
 &= \frac{1}{|\tilde{\omega}|} \int_{\tilde{\omega}} (\gamma(\bar{\mathbf{u}}) + e_{\tilde{\omega}}) : \mathbf{A}_{\tilde{\omega}} : (\gamma(\bar{\mathbf{u}}) + e_{\tilde{\omega}}),
 \end{aligned}$$

where we have utilized (35) in the third line. This proves (59).  $\square$

**Step vi.** The limit (59) in **Step v** holds for the entire sequence rather than only on the subsequence, which implies (34) according to (33).

**PROOF.** Suppose (59) does not hold for some sequence  $\mathbf{u}^\epsilon$ . Then there exists some  $c > 0$  and a subsequence of  $\mathbf{u}^\epsilon$ , still denoted as  $\mathbf{u}^\epsilon$ , such that

$$|J_\epsilon^*(\tilde{\omega}) - E^*| > c. \quad (67)$$

where  $E^*$  represents the RHS of (59). However, since the bound on  $e_{i||j}(\epsilon)$  in **Step i** still hold for such a subsequence, the result in (59) is true for some subsequence of this subsequence, namely,

$$\lim_{\epsilon \rightarrow 0} J_\epsilon^*(\tilde{\omega}) = E^*$$

holds for such some subsequence. As (35) has only one solution, both  $E^*$  are the same for these subsequences. This, however, contradicts with (67).  $\square$

## 4.2 The condition to achieve the upper bound of ADS

According to Theorem 2 in the main text, the ADS attains the upper bound if (35) has a zero solution, which means

$$\int_{\tilde{\omega}} \gamma(\bar{\mathbf{u}}) : \mathbf{A}_{\tilde{\omega}} : \gamma(\mathbf{v}) = - \int_{\tilde{\omega}} e_{\tilde{\omega}} : \mathbf{A}_{\tilde{\omega}} : \gamma(\mathbf{v}) = 0, \quad \forall \mathbf{v} \in \dot{\mathbf{V}}_\#(\tilde{\omega}). \quad (68)$$

We rewrite the RHS of above equation as

$$\int_{\tilde{\omega}} e_{\tilde{\omega}} : \mathbf{A}_{\tilde{\omega}} : \gamma(\mathbf{v}) = \int_{\tilde{\omega}} \boldsymbol{\sigma}_{\tilde{\omega}} : (\nabla \mathbf{v}_{\tilde{\omega}} - \mathbf{b} \mathbf{v}_3), \quad (69)$$

where  $\boldsymbol{\sigma}_{\tilde{\omega}} = \mathbf{A}_{\tilde{\omega}} : e_{\tilde{\omega}} = \sigma^{\alpha\beta} \mathbf{a}_\alpha \otimes \mathbf{a}_\beta$ , with components given by  $\sigma^{\alpha\beta} = a^{\alpha\beta\theta\tau} e_{\theta\tau}$ , denotes the membrane stress;  $\mathbf{b}$  represents the curvature tensor (second fundamental form) of  $\tilde{\omega}$ . Here, the symmetric gradient of  $\mathbf{v}_{\tilde{\omega}}$  appears in  $\gamma(\mathbf{v})$  can be replaced by  $\nabla \mathbf{v}_{\tilde{\omega}}$  because the stress tensor  $\boldsymbol{\sigma}_{\tilde{\omega}}$  is symmetric.

Now, we consider  $\forall \mathbf{v} \in H^1(\tilde{\omega})/\ker \gamma \subset \dot{V}_\#(\tilde{\omega})$  and suppose (68) holds. For the first term in RHS of (69), we have

$$\begin{aligned} \int_{\tilde{\omega}} \sigma_{\tilde{\omega}} : \nabla \mathbf{v}_{\tilde{\omega}} &= \int_{\tilde{\omega}} \operatorname{div} [\sigma_{\tilde{\omega}} \cdot \mathbf{v}_{\tilde{\omega}}] - \int_{\tilde{\omega}} [\operatorname{div} \sigma_{\tilde{\omega}}] \cdot \mathbf{v}_{\tilde{\omega}} \\ &= - \int_{\tilde{\omega}} [\operatorname{div} \sigma_{\tilde{\omega}}] \cdot \mathbf{v}_{\tilde{\omega}}, \end{aligned} \quad (70)$$

where we have utilized divergence theorem and the closed surface condition.

Since (68) holds for any  $\mathbf{v} \in H^1(\tilde{\omega})/\ker \gamma$ , it follows from (69) and (70) that

$$\begin{aligned} \operatorname{div} \sigma_{\tilde{\omega}} &= \mathbf{0}, \\ \sigma_{\tilde{\omega}} : \mathbf{b} &= 0. \end{aligned} \quad (71)$$

By definition, the divergence  $\operatorname{div} \sigma_{\tilde{\omega}}$  is computed as

$$[\operatorname{div} \sigma_{\tilde{\omega}}]^\alpha = \partial_\gamma \sigma^{\alpha\gamma} + \Gamma_{\gamma\beta}^\beta \sigma^{\alpha\gamma} + \Gamma_{\theta\tau}^\alpha \sigma^{\theta\tau}.$$

The three terms in the RHS of above equation are given by

$$\begin{aligned} \partial_\gamma \sigma^{\alpha\gamma} &= \lambda_0 \left\{ (\partial_\gamma a^{\alpha\gamma}) a^{\theta\tau} e_{\theta\tau} + a^{\alpha\gamma} (\partial_\gamma a^{\theta\tau}) e_{\theta\tau} + a^{\alpha\gamma} a^{\theta\tau} \partial_\gamma e_{\theta\tau} \right\} \\ &\quad + 2\mu \left\{ \partial_\gamma a^{\alpha\theta} a^{\gamma\tau} e_{\theta\tau} + a^{\alpha\theta} \partial_\gamma a^{\gamma\tau} e_{\theta\tau} + a^{\alpha\theta} a^{\gamma\tau} \partial_\gamma e_{\theta\tau} \right\} \\ \Gamma_{\gamma\beta}^\beta \sigma^{\alpha\gamma} &= \lambda_0 a^{\alpha\gamma} a^{\theta\tau} \Gamma_{\gamma\sigma}^\sigma e_{\theta\tau} + 2\mu a^{\alpha\theta} a^{\gamma\tau} \Gamma_{\gamma\sigma}^\sigma e_{\theta\tau} \\ \Gamma_{\theta\tau}^\alpha \sigma^{\theta\tau} &= \lambda_0 a^{\theta\tau} a^{\xi\eta} \Gamma_{\theta\tau}^\alpha e_{\xi\eta} + 2\mu a^{\theta\xi} a^{\tau\eta} \Gamma_{\theta\tau}^\alpha e_{\xi\eta}. \end{aligned}$$

The derivative of stress consists of two parts

(1) The terms involving  $\lambda_0$

$$\begin{aligned} \partial_\gamma a^{\alpha\gamma} a^{\theta\tau} e_{\theta\tau} &= - \left( a^{\alpha\sigma} \Gamma_{\sigma\gamma}^\gamma + a^{\gamma\sigma} \Gamma_{\sigma\gamma}^\alpha \right) a^{\theta\tau} e_{\theta\tau}, \\ a^{\alpha\gamma} \partial_\gamma a^{\theta\tau} e_{\theta\tau} &= - \left( a^{\theta\sigma} \Gamma_{\sigma\gamma}^\gamma + a^{\tau\sigma} \Gamma_{\sigma\gamma}^\theta \right) a^{\alpha\gamma} e_{\theta\tau}, \\ a^{\alpha\gamma} a^{\theta\tau} \partial_\gamma e_{\theta\tau} &= a^{\alpha\gamma} a^{\theta\tau} \left( e_{\sigma\tau} \Gamma_{\theta\gamma}^\sigma + e_{\theta\sigma} \Gamma_{\tau\gamma}^\sigma + b_{\gamma\theta} e_{3\tau} + b_{\gamma\tau} e_{3\theta} \right). \end{aligned}$$

(2) The terms involving  $\mu$

$$\begin{aligned} \partial_\gamma a^{\alpha\theta} a^{\beta\tau} e_{\theta\tau} &= - \left( a^{\alpha\sigma} \Gamma_{\sigma\gamma}^\theta + a^{\theta\sigma} \Gamma_{\sigma\gamma}^\alpha \right) a^{\beta\tau} e_{\theta\tau}, \\ a^{\alpha\theta} \partial_\gamma a^{\beta\tau} e_{\theta\tau} &= - \left( a^{\tau\sigma} \Gamma_{\sigma\gamma}^\gamma + a^{\gamma\sigma} \Gamma_{\sigma\gamma}^\tau \right) a^{\alpha\theta} e_{\theta\tau}, \\ a^{\alpha\theta} a^{\beta\tau} \partial_\gamma e_{\theta\tau} &= a^{\alpha\theta} a^{\beta\tau} \left( e_{\sigma\tau} \Gamma_{\theta\gamma}^\sigma + e_{\theta\sigma} \Gamma_{\tau\gamma}^\sigma + b_{\gamma\theta} e_{3\tau} + b_{\gamma\tau} e_{3\theta} \right). \end{aligned}$$

The above equations utilized the identity

$$\partial_\gamma e_{\theta\tau} = e_{\sigma\tau} \Gamma_{\theta\gamma}^\sigma + e_{\theta\sigma} \Gamma_{\tau\gamma}^\sigma + b_{\gamma\theta} e_{3\tau} + b_{\gamma\tau} e_{3\theta},$$

which can be verified from the following relations

$$\begin{aligned} \partial_\gamma e_{\theta\tau} &= \partial_\gamma \left( \varepsilon_{ij} \Pi_\theta^i \Pi_\tau^j \right) = \varepsilon_{ij} \left( \partial_\gamma \Pi_\theta^i \Pi_\tau^j + \Pi_\theta^i \partial_\gamma \Pi_\tau^j \right), \\ \partial_\gamma \Pi_\theta^i &= \partial_\gamma (\mathbf{e}^i \cdot \mathbf{a}_\theta) = \mathbf{e}^i \cdot \partial_\gamma \mathbf{a}_\theta = \mathbf{e}^i \cdot \left( \Gamma_{\theta\tau}^\beta \mathbf{a}_\beta + b_{\theta\tau} \mathbf{n} \right) \\ &= \Gamma_{\theta\tau}^\beta \Pi_\beta^i + b_{\theta\tau} \Pi_3^i. \end{aligned}$$

After the terms in same color cancel out, we obtain

$$\begin{aligned} [\operatorname{div} \sigma_{\tilde{\omega}}]^\alpha &= \lambda_0 a^{\alpha\gamma} a^{\theta\tau} (b_{\gamma\theta} e_{3\tau} + b_{\gamma\tau} e_{3\theta}) \\ &\quad + 2\mu a^{\alpha\theta} a^{\beta\tau} (b_{\gamma\theta} e_{3\tau} + b_{\gamma\tau} e_{3\theta}) \\ &= 2\lambda_0 b^{\alpha\tau} e_{3\tau} + 2\mu (b^{\alpha\tau} e_{3\tau} + 2Ha^{\alpha\theta} e_{3\theta}) \\ &= \left( (2\lambda_0 + 2\mu) b^{\alpha\theta} + 4\mu Ha^{\alpha\theta} \right) e_{3\theta}, \end{aligned} \quad (72)$$

where  $H$  denotes the mean curvature<sup>4</sup>. In matrix form (under the standard basis  $\{\mathbf{e}_i\}$ ), we can rewrite (72) as

$$\operatorname{div} \sigma_{\tilde{\omega}} = (2(\lambda_0 + \mu) \mathbf{b} + 4\mu H \mathbf{I}) P \boldsymbol{\varepsilon} \cdot \mathbf{n}.$$

For the another term in (71), we have

$$\begin{aligned} \sigma_{\tilde{\omega}} : \mathbf{b} &= \sigma^{\theta\tau} b_{\theta\tau} v_3 = 2(\lambda_0 H a^{\alpha\beta} + \mu b^{\alpha\beta}) e_{\alpha\beta} \\ &= 2(\lambda_0 H \mathbf{I} + \mu \mathbf{b}) : P \boldsymbol{\varepsilon} = 0. \end{aligned}$$

Since  $\mathbf{b}$  is inherently tangent on  $\tilde{\omega}$ , multiplication by the projection matrix  $P$  has no effect, thus (71) is simplified as

$$\begin{aligned} (2(\lambda_0 + \mu) \mathbf{b} + 4\mu H P) \boldsymbol{\varepsilon} \cdot \mathbf{n} &= \mathbf{0}, \\ 2(\lambda_0 H P + \mu \mathbf{b}) : \boldsymbol{\varepsilon} &= 0. \end{aligned} \quad (73)$$

On the contrary, if (73) is satisfied, then (68) holds for any  $\mathbf{v} \in H^1(\tilde{\omega})/\ker \gamma$ , this equality then extends to  $\dot{V}_\#(\tilde{\omega})$  due to density of  $H^1(\tilde{\omega})/\ker \gamma$  in  $\dot{V}_\#(\tilde{\omega})$  and the continuity of the linear form in the RHS of (68). Therefore, it must admit a zero solution and the ADS attains the upper bound by Theorem 2 in the main text.

### 4.3 The upper bound of ABM for general shell lattice

In this section, we will show that the ABM of TPMS serves as the upper bound for all periodic surfaces. Furthermore, we prove a more general result. Instead of considering only the shell with uniform thickness, we also take the shell with variable thickness into account. Additionally, we do not assume that  $\tilde{\omega}$  is a closed surface in  $\mathbb{T}^3$ .

For generality consideration, we make some minor changes to the definitions in Section 2 before proving our general result. We represent the bidirectional offset distances of  $\tilde{\omega}$  as two continuous function over  $\tilde{\omega}$ , denoted as  $h_\epsilon^+, h_\epsilon^- : \tilde{\omega} \rightarrow \mathbb{R}^+$ , which satisfy

$$h_\epsilon^+(y), h_\epsilon^-(y) \rightarrow 0 \text{ as } \epsilon \rightarrow 0, \forall y \in \tilde{\omega}.$$

Namely, we only require that the thickness tends to 0 as  $\epsilon \rightarrow 0$ , but we do not require the thickness to be uniform or decrease at a specific rate. The compactness of  $\tilde{\omega}$  is still necessary but we do not assume  $\tilde{\omega}$  to be closed surface, i.e.,  $\tilde{\omega}$  may have boundaries. We will see that the closed surface condition is unnecessary for deriving the upper bound.

As  $\tilde{\omega}$  remains compact, the finite charts  $(S_i, \boldsymbol{\psi}_i)_{i \in I}$  and partition  $\{\tilde{\omega}_m\}$  still exists. Then we redefine

$$\tilde{\Omega}^\epsilon := \{ \tilde{\mathbf{x}} \in \mathbb{T}^3 : \tilde{\mathbf{x}} = \tilde{\mathbf{y}} + x_3 \mathbf{n}(\tilde{\mathbf{y}}), x_3 \in (-h_\epsilon^-(\tilde{\mathbf{y}}), h_\epsilon^+(\tilde{\mathbf{y}})), \tilde{\mathbf{y}} \in \tilde{\omega} \},$$

which is a 3-manifold when  $\epsilon$  is sufficiently small. We can still equip it with charts  $(B_i^\epsilon, \Phi_i^\epsilon)_{i \in I}$ , which are redefined by

$$B_i^\epsilon = \{ \tilde{\mathbf{x}} \in \mathbb{T}^3 : \tilde{\mathbf{x}} = \tilde{\mathbf{y}} + x_3 \mathbf{n}(\tilde{\mathbf{y}}), x_3 \in (-h_\epsilon^-(\tilde{\mathbf{y}}), h_\epsilon^+(\tilde{\mathbf{y}})), \tilde{\mathbf{y}} \in S_i \}$$

and

$$\Phi_i^\epsilon : B_i^\epsilon \rightarrow \mathcal{V}_i^\epsilon, \tilde{\mathbf{y}} + x_3 \mathbf{n}(\tilde{\mathbf{y}}) \mapsto (\boldsymbol{\psi}_i(\tilde{\mathbf{y}}), x_3)$$

with  $\mathcal{V}_i^\epsilon := \{(y, x_3) : y \in \mathcal{U}_i, -h_\epsilon^-(y) < x_3 < h_\epsilon^+(y)\}$ . The partition  $\{\tilde{\Omega}_m^\epsilon\}$  and the corresponding parameter domain  $\{\Omega_m^\epsilon\}$  are defined accordingly, similar to the case of uniform thickness.

The strain and elastic tensor can be defined over  $\tilde{\Omega}^\epsilon$  same as before. In this case, the relation  $\rho_\epsilon(\tilde{\omega}) \sim 2\epsilon|\tilde{\omega}|$  does not hold. Therefore, we consider the following function

$$J_\epsilon(\mathbf{u}; \tilde{\omega}, h_\epsilon^+, h_\epsilon^-) := \frac{1}{|\tilde{\Omega}^\epsilon|} \int_{\tilde{\Omega}^\epsilon} (\boldsymbol{\varepsilon}(\mathbf{u}) + \mathbf{I}) : \mathbf{A} : (\boldsymbol{\varepsilon}(\mathbf{u}) + \mathbf{I}),$$

<sup>4</sup>Here, we have used identity  $a^{\alpha\beta} b_{\alpha\beta} = 2H$ .

we denote its minimal value as

$$J_\epsilon^*(\tilde{\omega}, h_\epsilon^+, h_\epsilon^-) := \min_{\mathbf{u} \in V_\#(\tilde{\Omega}^\epsilon)} J_\epsilon(\mathbf{u}; \tilde{\omega}, h_\epsilon^+, h_\epsilon^-). \quad (74)$$

The ABM is still defined as the ratio between  $E_\epsilon(\tilde{\omega}; \frac{1}{3}I)$  and volume fraction  $\rho(\tilde{\Omega}^\epsilon)$ , which equals to the following limit

$$K_A := \frac{1}{9} \lim_{\epsilon \rightarrow 0} J_\epsilon^*(\tilde{\omega}, h_\epsilon^+, h_\epsilon^-). \quad (75)$$

According to this definition, the ABM is defined for triplet  $(\tilde{\omega}, h_\epsilon^+, h_\epsilon^-)$  rather than only dependent on  $\tilde{\omega}$ . For brevity, we term it as the *ABM of shell lattice*  $(\tilde{\omega}, h_\epsilon^+, h_\epsilon^-)$ . The ABM of the surface we considered in the main text is a special case when  $h_\epsilon^+ = h_\epsilon^- = \epsilon$ . The key result in this section is the following theorem.

**THEOREM 2.** *The ABM of any shell lattice has an upper bound*

$$K_A \leq \frac{4}{9}(\lambda_0 + \mu). \quad (76)$$

**PROOF.** Consider the global smooth vector field  $\mathbf{w}$  whose local coordinate representation is<sup>5</sup>

$$\mathbf{w}_1 = 0, \quad \mathbf{w}_2 = 0, \quad \mathbf{w}_3 = -\frac{3\lambda + 2\mu}{\lambda + 2\mu} \mathbf{x}_3$$

on each chart  $(B_m^\epsilon, \Phi_m^\epsilon)$ , we have

$$e_{\alpha\parallel\beta}^\epsilon(\mathbf{w}) = w_3 b_{\alpha\beta}, \quad e_{\sigma\parallel 3}^\epsilon(\mathbf{w}) = 0, \quad e_{3\parallel 3}^\epsilon(\mathbf{w}) = -\frac{3\lambda + 2\mu}{\lambda + 2\mu}. \quad (77)$$

Next, we remove the translation of  $\mathbf{w}$  to construct  $\mathbf{w}^* := \mathbf{w} - \langle \mathbf{w} \rangle$ , where  $\langle \mathbf{w} \rangle$  denotes the component-wise volume average of vector field, given by

$$\langle \mathbf{w} \rangle := \left( \frac{1}{|\tilde{\Omega}^\epsilon|} \int_{\tilde{\Omega}^\epsilon} \hat{\mathbf{w}}_i \right) \mathbf{e}^i,$$

which is a constant vector field over  $\tilde{\Omega}^\epsilon$ . Thus  $\mathbf{w}^* \in V_\#(\tilde{\Omega}^\epsilon)$  and  $e_{i\parallel j}^\epsilon(\mathbf{w}^*) = e_{i\parallel j}^\epsilon(\mathbf{w})$ .

By definition (74), we have

$$\begin{aligned} J_\epsilon^*(\tilde{\omega}, h_\epsilon^+, h_\epsilon^-) &= \min_{\mathbf{u} \in V_\#(\tilde{\Omega}^\epsilon)} \frac{1}{|\tilde{\Omega}^\epsilon|} \int_{\tilde{\Omega}^\epsilon} (\epsilon(\mathbf{u}) + \mathbf{I}) : \mathbf{A} : (\epsilon(\mathbf{u}) + \mathbf{I}) d\tilde{\Omega}^\epsilon \\ &\leq \frac{1}{|\tilde{\Omega}^\epsilon|} \int_{\tilde{\Omega}^\epsilon} (\epsilon(\mathbf{w}) + \mathbf{I}) : \mathbf{A} : (\epsilon(\mathbf{w}) + \mathbf{I}) d\tilde{\Omega}^\epsilon \\ &= \frac{1}{|\tilde{\Omega}^\epsilon|} \sum_m \int_{\Omega_m^\epsilon} A^{ijkl,\epsilon} (e_{i\parallel j}^\epsilon(\mathbf{w}) + g_{ij}^\epsilon) (e_{k\parallel l}^\epsilon(\mathbf{w}) + g_{kl}^\epsilon) \sqrt{g}^\epsilon dx. \end{aligned} \quad (78)$$

The first inequality in (78) (second line) is from the condition of minimizer and  $e_{i\parallel j}^\epsilon(\mathbf{w}^*) = e_{i\parallel j}^\epsilon(\mathbf{w})$ .

Let

$$\tilde{h}_\epsilon := \sup_{\mathbf{y} \in \tilde{\omega}} \max \{ |h_\epsilon^-(\mathbf{y})|, |h_\epsilon^+(\mathbf{y})| \}.$$

Since  $h_\epsilon^-, h_\epsilon^+$  are continuous on compact manifold  $\tilde{\omega}$ , it satisfies  $|x_3| < \tilde{h}_\epsilon$  and  $\tilde{h}_\epsilon \rightarrow 0$  as  $\epsilon \rightarrow 0$ . Therefore, we have

$$\begin{aligned} g_{ij}^\epsilon &= a_{ij} + O(\tilde{h}_\epsilon), \\ g^{ij,\epsilon} &= a^{ij} + O(\tilde{h}_\epsilon), \\ \sqrt{g}^\epsilon &= a + O(\tilde{h}_\epsilon). \end{aligned}$$

<sup>5</sup>Although this definition is expressed on each chart, it can be easily verified that this vector field is globally well defined on  $\tilde{\Omega}^\epsilon$ .

Here, we utilized Lemma 2 (15), (16), (17), and (18). Although these relations are derived in the case of uniform thickness, it is clear that they are only dependent on the maximal thickness. Substitute these terms into (78) and apply Lemma 2 and 3, we have

$$\begin{aligned} J_\epsilon^*(\tilde{\omega}, h_\epsilon^+, h_\epsilon^-) &\leq \frac{1}{|\tilde{\Omega}^\epsilon|} \sum_m \int_{\Omega_m^\epsilon} A^{ijkl}(0) \left( e_{i\parallel j}^\epsilon(\mathbf{w}) + a_{ij} \right) \left( e_{k\parallel l}^\epsilon(\mathbf{w}) + a_{kl} \right) \sqrt{a} dx \\ &\quad + O(\tilde{h}_\epsilon). \end{aligned} \quad (79)$$

Next, we substitute (77) into (79) and obtain

$$\begin{aligned} J_\epsilon^*(\tilde{\omega}, h_\epsilon^+, h_\epsilon^-) &\leq \frac{1}{|\tilde{\Omega}^\epsilon|} \sum_m \left\{ \int_{\Omega_m^\epsilon} A^{\alpha\beta\theta\tau}(0) (w_3 b_{\theta\tau} + a_{\theta\tau}) (w_3 b_{\alpha\beta} + a_{\alpha\beta}) \sqrt{a} dx \right. \\ &\quad - 2 \int_{\Omega_m^\epsilon} A^{\alpha\beta 33}(0) (w_3 b_{\alpha\beta} + a_{\alpha\beta}) \frac{2\lambda}{\lambda + 2\mu} \sqrt{a} dx \\ &\quad \left. + \int_{\Omega_m^\epsilon} A^{3333}(0) \frac{2\lambda}{\lambda + 2\mu} \frac{2\lambda}{\lambda + 2\mu} \sqrt{a} dx \right\} + O(\tilde{h}_\epsilon) \\ &= \frac{1}{|\tilde{\Omega}^\epsilon|} \sum_m \int_{\Omega_m^\epsilon} 4(\lambda_0 + \mu) \sqrt{a} dx + O(\tilde{h}_\epsilon) \\ &= \frac{1}{|\tilde{\Omega}^\epsilon|} \sum_m \int_{\Omega_m^\epsilon} 4(\lambda_0 + \mu) \sqrt{g}^\epsilon dx + O(\tilde{h}_\epsilon) \\ &= \frac{1}{|\tilde{\Omega}^\epsilon|} \int_{\tilde{\Omega}^\epsilon} 4(\lambda_0 + \mu) d\tilde{\Omega}^\epsilon + O(\tilde{h}_\epsilon) = 4(\lambda_0 + \mu) + O(\tilde{h}_\epsilon), \end{aligned} \quad (80)$$

where the terms involving  $w_3$  are incorporated into  $O(\tilde{h}_\epsilon)$  in the first equality (fourth line), since  $|w_3| \leq (3\lambda + 2\mu)/(\lambda + 2\mu)|\tilde{h}_\epsilon|$ . Let  $\epsilon \rightarrow 0$  in (80), we have

$$\limsup_{\epsilon \rightarrow 0} J_\epsilon^*(\tilde{\omega}) \leq 4(\lambda_0 + \mu).$$

which, according to (75), implies (76).  $\square$

## 5 Semi-analytical evaluation of ADS for revolution surfaces

We consider the revolution surface around  $x$ -axis. Suppose its radius is given by a periodic function  $R : \mathbb{T} \rightarrow \mathbb{R}$ , then the surface is parameterized as

$$\mathbf{r}(x, \theta) = (x, R(x) \cos \theta, R(x) \sin \theta)^\top.$$

The covariant basis is given by

$$\begin{aligned} \mathbf{a}_x &= \partial_x \mathbf{r} = (1, R'(x) \cos \theta, R'(x) \sin \theta)^\top, \\ \mathbf{a}_\theta &= \partial_\theta \mathbf{r} = (0, -R(x) \sin \theta, R(x) \cos \theta)^\top. \end{aligned}$$

Due to the symmetry of revolution surfaces, the solution of (35) is rotational invariant w.r.t.  $x$ -axis, thus we express it as the following vector field

$$\mathbf{u} = \tau(x) \mathbf{a}_x + s(x) \mathbf{n}, \quad (81)$$

where  $\mathbf{n}$  denotes the normal vector;  $\tau$  and  $s$  are two periodic functions. As indicated by Remark 3, we substitute (81) into (37), and

get the following problem on parameter domain

$$E_A(\tilde{\omega}; \mathbf{e}^{11}) = \min_{s^\#, \tau^\#} \frac{1}{|\tilde{\omega}|} \int_{-1}^1 \int_0^{2\pi} c_0(x) + \mathbf{c}_1^\top(x) \boldsymbol{\eta}(x) + \boldsymbol{\eta}^\top(x) \mathbf{C}_2(x) \boldsymbol{\eta}(x) d\theta dx, \quad (82)$$

where  $\boldsymbol{\eta}(x) = (s(x), \tau(x), \tau'(x))^\top$ ;  $c_0$ ,  $\mathbf{c}_1$  and  $\mathbf{C}_2$  are some periodic scalar, vector, and matrix function of  $x$ , respectively. Note the integrand is independent of  $\theta$  due to the rotational symmetry of  $\tilde{\omega}$ , thus this integral is simplified to a 1D integral. We evenly divide the integral  $[-1, 1]$  into  $10^5$  segments. The function  $s, \tau$  are discretized as the values  $\{s_i\}$  and  $\{\tau_i\}$  on the nodes, with -1 and 1 regarded as the same node due to periodic condition, the derivative  $\tau'$  is discretized using central difference scheme. Then (82) is approximated by

$$E_A(\tilde{\omega}; \mathbf{e}^{11}) = \min_{s^h, \tau^h} \frac{1}{|\tilde{\omega}|} \sum_i 2\pi f_i^h(s^h, \tau^h) \Delta x, \quad (83)$$

where  $\Delta x = 2 \times 10^{-5}$  is the segment length and

$$f_i^h(s^h, \tau^h) = c_0^h(x_i) + [\mathbf{c}_1^h(x_i)]^\top \boldsymbol{\eta}_i + \boldsymbol{\eta}_i^\top \mathbf{C}_2(x_i) \boldsymbol{\eta}_i,$$

and

$$\boldsymbol{\eta}_i = \left( s_i, \tau_i, \frac{\tau_{i+1} - \tau_{i-1}}{2\Delta x} \right)^\top.$$

The objective in (83) is a quadratic function, thus the minimal value is found by assembling and solving a linear system.

## 6 Sensitivity of ADS with respect to perturbation

Let us introduce a simple example to illustrate how sensitive ADS could be and why geometry approximation could seriously impacts the ADS. Consider a infinite plane  $z = 0$ , which is definitely a periodic surface and thus considered as a submanifold  $\mathbb{T}^2 \subset \mathbb{T}^3$ . The ADS of  $\mathbb{T}^2$  under planar stretch strain  $\mathbf{e}^{11}$  is

$$E_A(\mathbb{T}^2; \mathbf{e}^{11}) = \lambda_0 + 2\mu.$$

However, if we only perturb this surface slightly through offsetting it normally by a small distance  $h(x, y) := \delta \cos(k\pi x)$ , where  $\delta$  is a small positive constant and  $k$  denotes a non-zero integer, the ADS under strain  $\mathbf{e}^{11}$  suddenly reduces to zero, i.e., we have

$$E_A(\mathbb{T}_\delta^2; \mathbf{e}^{11}) = 0,$$

where  $\mathbb{T}_\delta^2$  denotes the perturbed surface. This holds for arbitrarily small  $\delta$  and any  $k$ , as demonstrated by the following proposition

**PROPOSITION 1.** *For  $\mathbb{T}^2$  and perturbed surface  $\mathbb{T}_\delta^2$ , we have*

$$E_A(\mathbb{T}^2; \mathbf{e}^{11}) = \lambda_0 + 2\mu,$$

$$E_A(\mathbb{T}_\delta^2; \mathbf{e}^{11}) = 0,$$

where  $\mathbb{T}_\delta^2 = \{(x, y, z) \in \mathbb{T}^3 : z = \delta \cos(k\pi x)\}$  for any  $\delta > 0$  and  $k \in \mathbb{Z} \setminus \{0\}$ .

**PROOF.** If  $\tilde{\omega} = \mathbb{T}^2$ , the RHS of (35) evaluates to

$$\begin{aligned} - \int_{\mathbb{T}^2} \mathbf{e}^{11} : \mathbf{A}_{\tilde{\omega}} : \text{Sym}[\nabla \mathbf{v}_{\tilde{\omega}}] &= - \int_{\mathbb{T}^2} (\lambda_0 + 2\mu) \partial_x v_x + \lambda_0 \partial_y v_y \\ &= 0, \quad \forall \mathbf{v} \in \mathbf{H}^1(\tilde{\omega}). \end{aligned}$$

Thus the solution of (35) is zero, and we have

$$E_A(\tilde{\omega}; \mathbf{e}^{11}) = E_M(\tilde{\omega}; \mathbf{e}^{11}) = \lambda_0 + 2\mu$$

according to Theorem 2 in the main text.

If  $\tilde{\omega} = \mathbb{T}_\delta^2$ , we consider the following parameterization for brevity

$$\mathbf{r} = (x, y, \delta \cos(k\pi x))^\top.$$

The local covariant basis is given by

$$\mathbf{g}_1 = \partial_x \mathbf{r} = (1, 0, -k\pi \delta \sin(k\pi x))^\top,$$

$$\mathbf{g}_2 = \partial_y \mathbf{r} = (0, 1, 0)^\top.$$

The covariant components of the second fundamental form under this basis is computed as

$$\mathbf{b} = \begin{pmatrix} -\frac{k^2 \pi^2 \delta \cos(k\pi x)}{\sqrt{1+k^2 \pi^2 \delta^2 \sin^2(k\pi x)}} & 0 \\ 0 & 0 \end{pmatrix}$$

and the projected macro-strain  $\mathbf{e}_{\tilde{\omega}}$  is given by

$$\mathbf{e}_{\tilde{\omega}} = \begin{pmatrix} 1 & 0 \\ 0 & 0 \end{pmatrix}.$$

Therefore, we construct a vector field  $\mathbf{u}$  such that

$$\mathbf{u}_{\tilde{\omega}} = 0, \quad u_3 = \frac{1}{b_{11}}.$$

Clearly,  $\mathbf{u}$  is periodic. Then we have

$$\gamma(\mathbf{u}) + \mathbf{e}_{\tilde{\omega}} = -u_3 \mathbf{b} + \mathbf{e}_{\tilde{\omega}} = \mathbf{0}.$$

This means  $\mathbf{u}$  is exactly the solution of (35) and the ADS integral (34) reduces to zero. The only problem is that  $\mathbf{u} \notin \mathbf{H}^1(\tilde{\omega})$ , as it tends to infinity very fast near the points where  $k\pi x = \pm \frac{1}{2}\pi + m\pi$ ,  $m \in \mathbb{Z}$ . However, given that  $|\mathbf{u}|_{\tilde{\omega}} \lesssim |\gamma(\mathbf{u})|_{L^2(\tilde{\omega})} = |\mathbf{e}_{\tilde{\omega}}|_{L^2(\tilde{\omega})} < \infty^6$ , we have  $\mathbf{u} \in \dot{\mathbf{V}}_\#(\tilde{\omega})$ , namely, it belongs to the extended space after the completion.  $\square$

This proposition implies that even an infinitesimally small error in the geometry could lead to a significant change in the ADS. With such sensitivity, one can hardly guarantee that a discretization scheme could yield a converged solution to the analytical one.

## 7 Integral on $SO(3)$

To calculate above integral, we utilize the parameterization with Euler angles:

$$\mathbf{R} : (0, 2\pi) \times (0, \pi) \times (0, 2\pi) \rightarrow SO(3), \quad (\alpha, \beta, \gamma) \mapsto R_z(\alpha) R_y(\beta) R_z(\gamma),$$

where  $R_y, R_z$  denote the rotations around corresponding axes. The unique Haar measure over  $SO(3)$  is given by

$$d\mu = \sin \beta \, d\alpha \, d\beta \, d\gamma.$$

Therefore, we rewrite  $f_s(\mathbf{C}_A)$  as

$$f_s(\mathbf{C}_A) = \int_0^{2\pi} \int_0^\pi \int_0^{2\pi} [\boldsymbol{\varepsilon}(\mathbf{R})]^\top [\mathbf{C}_A] [\boldsymbol{\varepsilon}(\mathbf{R})] \sin \beta \, d\alpha \, d\beta \, d\gamma,$$

where  $[\cdot]$  denotes the Voigt representation. After computation, we obtain the compact form in the main text (with a constant scaling).

<sup>6</sup>The symbol ' $\lesssim$ ' means 'less than or equal to up to a constant'.

## 8 Time derivative in normal flow

Suppose the middle surface  $\tilde{\omega}$  undergoes a normal velocity  $v_n : \tilde{\omega} \rightarrow \mathbb{R}$ , we can verify the following time derivatives

$$\begin{aligned} \dot{a}^{\alpha\beta} &= 2v_n b^{\alpha\beta}, \quad \dot{b}_{\alpha\beta} = \partial_{ij}v_n - v_n c_{ij} - \partial_k v_n \Gamma_{ij}^k, \\ \dot{\Gamma}_{\alpha\beta}^\sigma &= -v_n b_\beta^\sigma|_\alpha - b_\alpha^\sigma \partial_\beta v_n - b_\beta^\sigma \partial_\alpha v_n + g^{\sigma\theta} b_{\alpha\beta} \partial_\theta v_n, \\ \sqrt{\det a} &= -2v_n H \sqrt{\det a}, \end{aligned} \quad (84)$$

where  $c_{ij}$  is the third fundamental form, and  $b_\beta^\sigma|_\alpha$  denotes the co-variant derivative of the curvature tensor, computed as

$$b_\beta^\sigma|_\alpha = \partial_\alpha b_\beta^\sigma + \Gamma_{\alpha\tau}^\sigma b_\beta^\tau - \Gamma_{\beta\alpha}^\tau b_\tau^\sigma.$$

For a time dependent integrand defined on  $\tilde{\omega}(t)$ , the time derivative of its integral is

$$\frac{d}{dt} \int_{\tilde{\omega}(t)} f(t) = \int_{\tilde{\omega}(t)} \dot{f}(t) - \int_{\tilde{\omega}(t)} 2v_n H f(t). \quad (85)$$

For the surface area  $A := |\tilde{\omega}|$ , the derivative is  $\dot{A} = - \int_{\tilde{\omega}} 2v_n H$ .

The formulation in Proposition 2 is derived as follows

PROOF. According to (85), the time derivative of the integral in ADS is

$$\begin{aligned} \dot{I}_a^s &= \int_{\tilde{\omega}} (\gamma(\tilde{\mathbf{u}}) + e_{\tilde{\omega}}) : (\dot{\mathbf{A}}_{\tilde{\omega}} - 2v_n H \mathbf{A}_{\tilde{\omega}}) : (\gamma(\tilde{\mathbf{u}}) + e_{\tilde{\omega}}) \\ &\quad + \int_{\tilde{\omega}} 2(\gamma(\tilde{\mathbf{u}}) + e_{\tilde{\omega}}) : \mathbf{A}_{\tilde{\omega}} : \frac{d}{dt} (\gamma(\tilde{\mathbf{u}}) + e_{\tilde{\omega}}). \end{aligned} \quad (86)$$

From (84) and the definition of tensor  $\mathbf{A}_{\tilde{\omega}}$ , the time derivative  $\dot{\mathbf{A}}_{\tilde{\omega}}$  is given by

$$\dot{a}^{\alpha\beta\theta\tau} = 2v_n B^{\alpha\beta\theta\tau},$$

where

$$B^{\alpha\beta\theta\tau} := \lambda_0(b^{\alpha\beta} a^{\theta\tau} + a^{\alpha\beta} b^{\theta\tau}) + \mu(b^{\alpha\theta} a^{\beta\tau} + a^{\alpha\theta} b^{\beta\tau} + b^{\alpha\tau} a^{\beta\theta} + a^{\alpha\tau} b^{\beta\theta}).$$

For the second integral in (86), we abbreviate the time derivative as

$$\eta(\tilde{\mathbf{u}}, v_n) := \frac{d}{dt} \gamma(\tilde{\mathbf{u}}) + \frac{d}{dt} e_{\tilde{\omega}},$$

which is a second-order tensor. The time derivative of the membrane strain is

$$\frac{d}{dt} \gamma_{\alpha\beta}(\tilde{\mathbf{u}}) = \gamma_{\alpha\beta}(\dot{\tilde{\mathbf{u}}}) - \dot{\Gamma}_{\alpha\beta}^\theta \tilde{u}_\theta - \dot{b}_{\alpha\beta} \tilde{u}_3.$$

The time derivative of  $e_{\tilde{\omega}}$  is

$$\frac{d}{dt} e_{\tilde{\omega}} = \frac{d}{dt} (P_\varepsilon P^\top) = \dot{P}_\varepsilon P^\top + P_\varepsilon \dot{P}^\top,$$

where

$$\dot{P} = -\dot{\mathbf{n}}\mathbf{n}^\top - \mathbf{n}\dot{\mathbf{n}}^\top$$

and  $\dot{\mathbf{n}} = -\nabla v_n$ . We utilize the variational equation (35) to eliminate  $\gamma(\dot{\tilde{\mathbf{u}}})$ , the remaining terms are

$$\eta(\tilde{\mathbf{u}}, v_n) \rightarrow -\dot{\Gamma}_{\alpha\beta}^\theta \tilde{u}_\theta - \dot{b}_{\alpha\beta} \tilde{u}_3 + 2\text{Sym}[P_\varepsilon \mathbf{n} \nabla v_n^\top],$$

where we have used the relation  $\sigma : P_\varepsilon \nabla v_n \mathbf{n}^\top = 0$ , which holds for any second-order tensor  $\sigma$  in the tangent space. According to (84), the terms  $-\dot{\Gamma}_{\alpha\beta}^\theta \tilde{u}_\theta$  and  $-\dot{b}_{\alpha\beta} \tilde{u}_3$  are exactly the components of the following tensors

$$\begin{aligned} -\dot{\Gamma}_{\alpha\beta}^\theta \tilde{u}_\theta &\rightarrow v_n \tilde{\mathbf{u}}_{\tilde{\omega}} \cdot \nabla \mathbf{b} + 2\text{Sym}[\mathbf{b} \tilde{\mathbf{u}}_{\tilde{\omega}} \nabla v_n^\top] - (\tilde{\mathbf{u}}_{\tilde{\omega}} \cdot \nabla v_n) \mathbf{b} \\ -\dot{b}_{\alpha\beta} \tilde{u}_3 &\rightarrow -\tilde{\mathbf{u}}_3 \nabla^2 v_n + (v_n \tilde{\mathbf{u}}_3) \mathbf{c}, \end{aligned}$$

where  $\mathbf{c}$  denotes the third fundamental form. Finally, we obtain the formula in Proposition 2.  $\square$

## A Proof of Theorem 4

(a), (b), (c) have been established in [Ciarlet and Lods 1996; Ciarlet et al. 1996]. We provide basically the same proof here for completeness.

For (a), we utilize Cauchy-Schwarz inequality and get

$$\begin{aligned} \int_{U_m} |\tilde{f}|^2 ds &= \int_{U_m} \frac{1}{4} \left| \int_{-1}^1 f dx_3 \right|^2 ds \leq \frac{1}{2} \int_{U_m} \int_{-1}^1 |f|^2 dx_3 ds \\ &= \frac{1}{2} \int_{\Omega_m} |f|^2 dx, \end{aligned}$$

hence  $\|\tilde{f}\|_{0,U_m} \leq \frac{1}{\sqrt{2}} \|f\|_{0,\Omega_m}$ .

For (b), we consider an arbitrary function  $\tilde{\varphi} \in \mathcal{D}(U_m)$ , let  $\varphi : \Omega_m \rightarrow \mathbb{R}$  be defined by  $\varphi(y, x_3) = \tilde{\varphi}(y)$  for  $(y, x_3) \in \Omega_m$ . Then we have

$$\int_{\Omega} f \partial_\alpha \varphi dx = - \int_{\Omega} \partial_\alpha f \varphi dx$$

by Green's formula. Since  $\varphi$  and  $\partial_\alpha \varphi$  are independent of  $x_3$ , Fubini theorem gives

$$\int_{U_m} \tilde{f} \partial_\alpha \tilde{\varphi} ds = - \int_{U_m} \overline{\partial_\alpha f} \tilde{\varphi} ds$$

hence  $\tilde{f} \in H^1(U_m)$  and  $\partial_\alpha \tilde{f} = \overline{\partial_\alpha f}$ . Apply the result in (a) on  $f$  and its derivative, we get  $\|\tilde{f}\|_{1,U_m} \leq \frac{1}{\sqrt{2}} \|f\|_{1,\Omega_m}$ .

For (c), given  $f \in \mathcal{C}^1(\overline{\Omega_m})$ , an integration by part yields

$$\int_{-1}^1 x_3 f(y, x_3) dx_3 = \frac{1}{2} \int_{-1}^1 (1 - x_3^2) \partial_3 f(y, x_3) dx_3 \quad \text{for all } y \in \tilde{\omega}.$$

From (a) and (b), we know the mappings  $f \in H^1(\Omega_m) \mapsto \tilde{f} \in H^1(U_m)$  and  $f \in L^2(\Omega_m) \mapsto \tilde{f} \in L^2(U_m)$  are both continuous. Hence, above formula also holds for  $f \in H^1(\Omega_m)$ .

For (d), we note that in the overlapped region of distinct charts of  $\tilde{\Omega}^\varepsilon$ , their  $x_3$  coordinates are the same. Therefore,  $\tilde{f}$  is well defined. We consider the relation

$$\begin{aligned} \|\tilde{f}\|_{H^1(\tilde{\omega})}^2 &= \sum_m \int_{U_m} (|\tilde{f}|^2 + a^{\alpha\beta} \partial_\alpha \tilde{f} \partial_\beta \tilde{f}) \sqrt{a} dy \\ &\leq C \sum_m \|\tilde{f}\|_{1,U_m}^2 \leq \frac{C}{2} \sum_m \|f\|_{1,\Omega_m}^2, \end{aligned}$$

where the first inequality comes from the boundness of metric  $a^{\alpha\beta}$  and area element  $\sqrt{a}$ ; the second inequality holds due to the results in (b). Then we have the following inequality

$$\sum_m \|f\|_{1,\Omega_m}^2 \leq C \sum_m \int_{\Omega_m} (f^2 + g^{ij}(\epsilon) \partial_i f \partial_j f) \sqrt{g(\epsilon)} dx = \frac{C}{\epsilon} \|f\|_{1,\tilde{\Omega}^\varepsilon}^2,$$

where the first inequality comes from the positive definiteness of metric  $g^{ij,\epsilon}$  and the positive lower bound of volume element  $\sqrt{g(\epsilon)}$ . Hence, we have  $\|\tilde{f}\|_{H^1(\tilde{\omega})} \leq \frac{C}{\sqrt{\epsilon}} \|f\|_{1,\tilde{\Omega}^\varepsilon}$ .

## B Proof of Lemma 5

PROOF. Suppose the inequality does not hold, then there exists a sequence  $\epsilon_k$  and  $\mathbf{v}^k = (v_i^k) \in V_\#(\tilde{\Omega}^\epsilon)$  such that

$$\epsilon_k \rightarrow 0 \quad \text{as } k \rightarrow \infty,$$

$$\sum_m \sum_i \|v_{i,m}^k(\epsilon_k)\|_{1,\mathcal{V}_m}^2 = 1 \quad \text{for all } k, \quad (87)$$

$$\frac{1}{\epsilon_k} e_{i||j,m}(\epsilon_k)(\mathbf{v}_m^k) \rightarrow 0 \text{ in } L^2(\mathcal{V}_m) \text{ as } k \rightarrow \infty, \text{ for all } m, \quad (88)$$

where  $\mathbf{v}_m^k$  is the restriction of  $\mathbf{v}^k$  on  $B_m^\epsilon$  and  $v_{i,m}^k$  is its component under basis  $\{\mathbf{g}^{i,\epsilon}\}$ .

From (87), we know there exists a subsequence, denoted as  $\{\mathbf{v}_{i,m}^n(\epsilon_n)\}$ , such that

$$v_{i,m}^n(\epsilon_n) \rightarrow v_{i,m} \text{ in } H^1(\mathcal{V}_m), \quad v_{i,m}^n(\epsilon_n) \rightarrow v_{i,m} \text{ in } L^2(\mathcal{V}_m) \text{ as } n \rightarrow \infty. \quad (89)$$

The second convergence result is from Rellich–Kondrachov theorem.

From (88), we know

$$\frac{1}{\epsilon_n} \partial_3 e_{\alpha||\beta,m}(\epsilon_n)(\mathbf{v}_m^n) \rightarrow 0 \quad \text{in } H^{-1}(\mathcal{V}_m). \quad (90)$$

This is deduced by the definition of  $H^{-1}$  norm as follows

$$\begin{aligned} & \left\| \frac{1}{\epsilon_n} \partial_3 e_{\alpha||\beta,m}(\epsilon_n)(\mathbf{v}_m^n) \right\|_{-1,\mathcal{V}_m} \\ &= \sup_{\phi \in H_0^1(\mathcal{V}_m), \|\phi\|_{1,\mathcal{V}_m}=1} \left| \int_{\mathcal{V}_m} \frac{1}{\epsilon_n} \partial_3 e_{\alpha||\beta,m}(\epsilon_n)(\mathbf{v}_m^n) \cdot \phi \right| \\ &= \sup_{\substack{\phi \in H_0^1(\mathcal{V}_m), \\ \|\phi\|_{1,\mathcal{V}_m}=1}} \left| \int_{\mathcal{V}_m} \frac{1}{\epsilon_n} e_{\alpha||\beta,m}(\epsilon_n)(\mathbf{v}_m^n) \cdot \partial_3 \phi \right| \\ &\leq \left\| \frac{1}{\epsilon_n} e_{\alpha||\beta,m}(\epsilon_n)(\mathbf{v}_m^n) \right\|_{0,\mathcal{V}_m} \rightarrow 0. \end{aligned}$$

On the other hand, we apply lemma 3.2 in [Ciarlet et al. 1996] that gives the following inequality

$$\begin{aligned} & \left\| \rho_{\alpha\beta}(\mathbf{v}_m^n) + \frac{1}{\epsilon_n} \partial_3 e_{\alpha||\beta,m}(\epsilon_n)(\mathbf{v}_m^n) \right\|_{-1,\mathcal{V}_m} \\ &\leq \left( \sum_i \|e_{i||3,m}(\epsilon_n)(\mathbf{v}_m^n)\|_{0,\mathcal{V}_m} \right. \\ &\quad \left. + \epsilon_n \sum_\alpha \|v_{\alpha,m}^n(\epsilon_n)\|_{0,\mathcal{V}_m} + \epsilon_n \|v_{3,m}^n(\epsilon_n)\|_{1,\mathcal{V}_m} \right). \end{aligned} \quad (91)$$

where  $\rho_{\alpha\beta}(\mathbf{v}_m^n)$  denotes the change of curvature when the shell undergoes a displacement  $\mathbf{v}_m^n$ , computed as

$$\begin{aligned} \rho_{\alpha\beta}(\mathbf{v}_m^n) &:= \partial_{\alpha\beta} v_{3,m}^n - \Gamma_{\alpha\beta}^\sigma \partial_\sigma v_{3,m}^n + b_\beta^\sigma (\partial_\alpha v_{\sigma,m}^n - \Gamma_{\alpha\sigma}^\tau v_{\tau,m}^n) \\ &\quad + b_\alpha^\sigma (\partial_\beta v_{\sigma,m}^n - \Gamma_{\beta\sigma}^\tau v_{\tau,m}^n) + b_\alpha^\sigma b_\beta^\tau v_{\sigma\tau,m}^n - c_{\alpha\beta} v_{3,m}^n. \end{aligned}$$

We apply (87) and (88) in (91) and obtain

$$\left\| \rho_{\alpha\beta}(\mathbf{v}_m^n) + \frac{1}{\epsilon_n} \partial_3 e_{\alpha||\beta,m}(\epsilon_n)(\mathbf{v}_m^n) \right\|_{-1,\mathcal{V}_m} \rightarrow 0 \quad \text{as } n \rightarrow \infty.$$

This combined with (90) implies

$$\rho_{\alpha\beta}(\mathbf{v}_m^n) \rightarrow 0 \quad \text{in } H^{-1}(\mathcal{V}_m) \quad \text{as } n \rightarrow \infty. \quad (92)$$

Next, we apply lemma 3.3 of [Ciarlet et al. 1996] according to (88), (89), and (92), which yields the following results on  $\mathcal{V}_m$

$$\mathbf{v}_m = (v_{i,m}) \text{ is independent of } x_3,$$

$$\gamma_{\alpha\beta}(\mathbf{v}_m) = \rho_{\alpha\beta}(\mathbf{v}_m) = 0, \quad (93)$$

$$v_{i,m}^n(\epsilon_n) \rightarrow v_{i,m} \quad \text{in } H^1(\mathcal{V}_m) \text{ as } n \rightarrow \infty. \quad (94)$$

Let  $\bar{\mathbf{v}}_m$  be a vector field on  $S_m$ , defined as

$$\bar{\mathbf{v}}_m := \overline{v_{i,m}} \mathbf{a}^i$$

where  $\overline{v_{i,m}}$  is the normal average defined as in Lemma 4. Since  $v_{i,m}$  is independent of  $x_3$ , this average is exactly itself. Therefore,  $\bar{\mathbf{v}}_m$  still satisfies (93) on  $\mathcal{U}_m$ , i.e.,

$$\gamma_{\alpha\beta}(\bar{\mathbf{v}}_m) = \rho_{\alpha\beta}(\bar{\mathbf{v}}_m) = 0 \quad \text{on } \mathcal{U}_m \quad (95)$$

Then, we apply the rigid displacement lemma [Bernadou et al. 1994] based on (95), which gives the following result

$$\bar{\mathbf{v}}_m = \mathbf{c}_m + \mathbf{d}_m \times \mathbf{r}_m \quad \text{a.e. } S_m,$$

where  $\mathbf{c}_m, \mathbf{d}_m \in \mathbb{R}^3$  are constant vectors; This means  $\bar{\mathbf{v}}_m$  is a rigid motion on  $S_m$ , this also holds on other charts. Note that these rigid motions on different charts coincide on their overlapped region. To show this, we consider the following identity

$$\mathbf{v} = v_{i,m}(\epsilon) \mathbf{g}_m^i(\epsilon) = v_{i,n}(\epsilon) \mathbf{g}_n^i(\epsilon), \quad \text{on } S_m \cap S_n.$$

Let  $\epsilon \rightarrow 0$  in above equation and using Lemma 2 and (89), we get

$$v_{i,m} \mathbf{a}_m^i = v_{j,n} \mathbf{a}_n^j.$$

Since  $v_{i,m}$  and  $v_{i,n}$  are independent of  $x_3$ , we obtain  $\bar{\mathbf{v}}_m = \bar{\mathbf{v}}_n$ . Consequently, the rigid motions on all charts are the same, denoted as  $\bar{\mathbf{v}}$ .

Suppose  $\mathbf{R} \in \ker \mathcal{E}(\cdot)$  is a arbitrary rigid motion on  $\tilde{\Omega}^\epsilon$ , then we have

$$\langle \mathbf{v}^k, \mathbf{R} \rangle_{L^2(\tilde{\Omega}^\epsilon)} = 0 \quad (96)$$

since  $\mathbf{v}^k \in V_\#(\tilde{\Omega}^\epsilon)$ . We denote  $R_i(\epsilon) = \mathbf{R} \cdot \mathbf{g}_i(\epsilon)$  and  $R_i = \mathbf{R} \cdot \mathbf{a}_i$ , then we have

$$R_\alpha(\epsilon) = R_i - \epsilon x_3 b_\alpha^\beta a_\beta^i, \quad R_3(\epsilon) = R_3.$$

Thus we derive the following limit

$$\begin{aligned} \frac{1}{\epsilon} \langle \mathbf{v}^k, \mathbf{R} \rangle_{L^2(\tilde{\Omega}^\epsilon)} &= \sum_m \int_{\Omega_m} v_{i,m}^k(\epsilon) R_i(\epsilon) g^{ij}(\epsilon) \sqrt{g(\epsilon)} dx \\ &\rightarrow \sum_m \int_{\Omega_m} v_{i,m} R_i a^{ij} \sqrt{a} dx \\ &= 2 \sum_m \int_{U_m} \overline{v_{i,m}} R_i a^{ij} \sqrt{a} ds \\ &= 2 \langle \bar{\mathbf{v}}, \mathbf{R} \rangle_{L^2(\tilde{\omega})}. \end{aligned}$$

According to (96), this limit equals zero, i.e., we have

$$\langle \bar{\mathbf{v}}, \mathbf{R} \rangle_{L^2(\tilde{\omega})} = 0$$

for an arbitrary rigid motion on  $\tilde{\omega}$ . Consequently, we get  $\bar{\mathbf{v}} = 0$ . However, considering the limit in (94), this contradicts (87).  $\square$

## References

- Grégoire Allaire. 2002. *Shape Optimization by the Homogenization Method* (1 ed.). Springer New York, NY. XVI, 458 pages. <https://doi.org/10.1007/978-1-4684-9286-6>
- M. Bernadou, P. G. Ciarlet, and B. Miara. 1994. Existence theorems for two-dimensional linear shell theories. *Journal of Elasticity* 34, 2 (01 Feb 1994), 111–138.
- Philippe G. Ciarlet and Véronique Lods. 1996. Asymptotic analysis of linearly elastic shells. I. Justification of membrane shell equations. *Archive for Rational Mechanics and Analysis* 136, 2 (01 Dec 1996), 119–161.
- Philippe G. Ciarlet, Véronique Lods, and Bernadette Miara. 1996. Asymptotic analysis of linearly elastic shells. II. Justification of flexural shell equations. *Archive for Rational Mechanics and Analysis* 136, 2 (01 Dec 1996), 163–190.
- Emmanuel Hebey. 1996. *Sobolev Spaces on Riemannian Manifolds* (1 ed.). Springer Berlin, Heidelberg. XII, 120 pages. Springer Book Archive.
- Julian Panetta, Qingnan Zhou, Luigi Malomo, Nico Pietroni, Paolo Cignoni, and Denis Zorin. 2015. Elastic textures for additive fabrication. *ACM Trans. Graph.* 34, 4, Article 135 (jul 2015), 12 pages. <https://doi.org/10.1145/2766937>
